# Supplementary material for: Proximity effects in graphene on monolayers of transition-metal phosphorus trichalcogenides MPX$_3$
Source: arXiv:2204.10524 source file (2022-07-21)
Supplement: Supplementary file 1 [file suppl.pdf]

# Supplemental Material: Proximity effects in graphene on monolayers of transition-metal phosphorus trichalcogenides $\text{MPX}_3$

Klaus Zollner<sup>1,\*</sup> and Jaroslav Fabian<sup>1</sup>

<sup>1</sup>*Institute for Theoretical Physics, University of Regensburg, 93040 Regensburg, Germany*

In the Supplemental Material we show the band structures, density of states, and fit results for the remaining heterostructures not shown in the main text. More specifically we show additional results for graphene on  $\text{MnPS}_3$ ,  $\text{NiPS}_3$ ,  $\text{FePS}_3$ ,  $\text{CoPS}_3$ ,  $\text{MnPSe}_3$ ,  $\text{NiPSe}_3$ ,  $\text{FePSe}_3$ , and  $\text{CoPSe}_3$ , where each  $\text{MPX}_3$  monolayer can be in the ferromagnetic, the antiferromagnetic Néel, the antiferromagnetic zigzag, and the antiferromagnetic stripy phase.

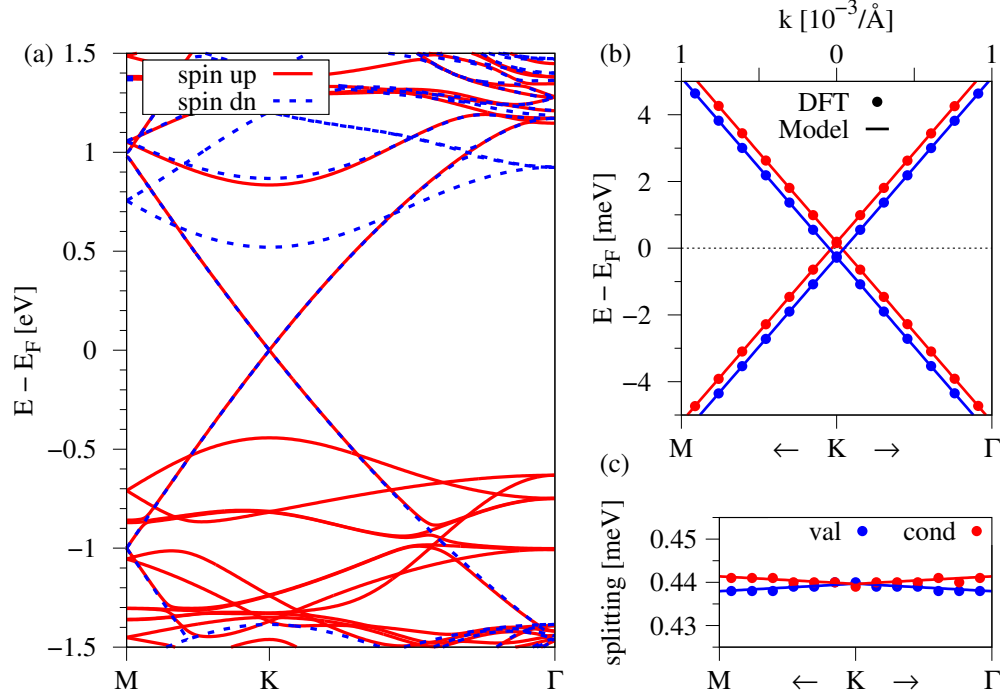

FIG. S1. (a) DFT-calculated band structure of the  $\text{graphene}/\text{MnPSe}_3$  heterostructure along the high-symmetry path M-K- $\Gamma$  without SOC, when the  $\text{MnPSe}_3$  is in the **ferromagnetic phase**. Red solid (blue dashed) lines correspond to spin up (spin down). (b) Zoom to the DFT-calculated (symbols) low energy Dirac bands near the K point with a fit to the model Hamiltonian (solid line). (c) The splitting of valence and conduction band.

\* klaus.zollner@physik.uni-regensburg.de

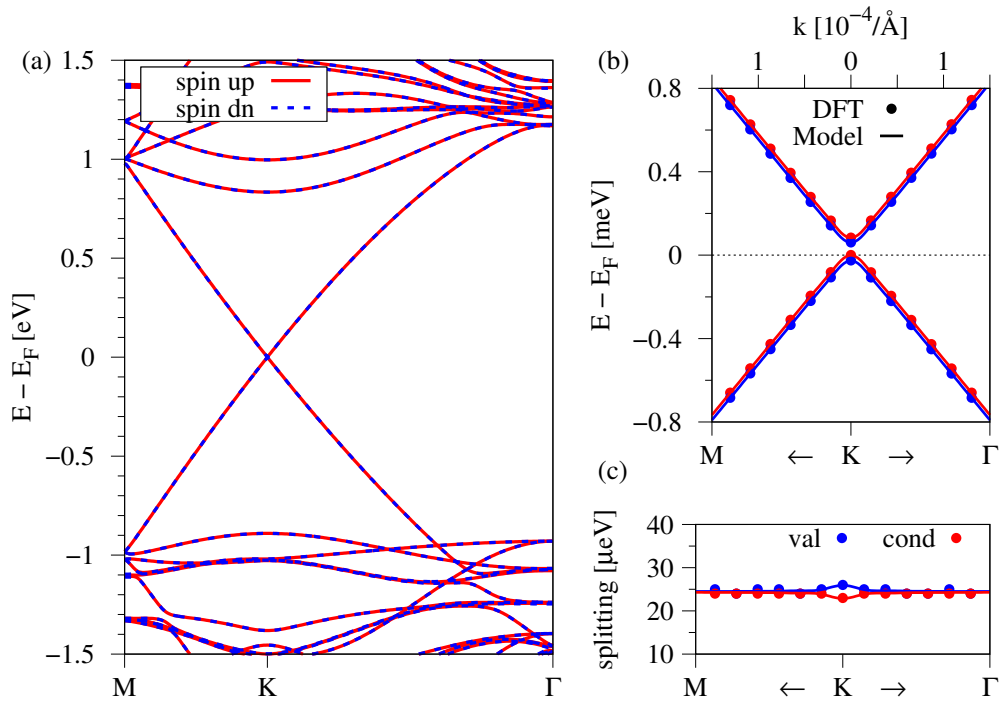

FIG. S2. (a) DFT-calculated band structure of the **graphene/MnPSe<sub>3</sub>** heterostructure along the high-symmetry path M-K- $\Gamma$  without SOC, when the MnPSe<sub>3</sub> is in the **antiferromagnetic Néel phase**. Red solid (blue dashed) lines correspond to spin up (spin down). (b) Zoom to the DFT-calculated (symbols) low energy Dirac bands near the K point with a fit to the model Hamiltonian (solid line). (c) The splitting of valence and conduction band.

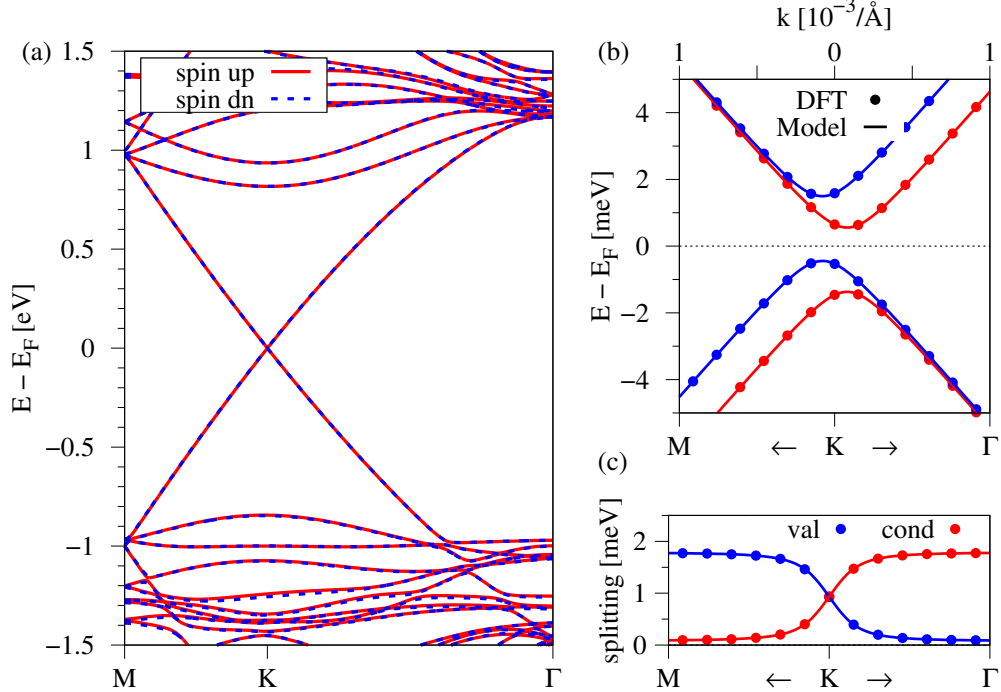

FIG. S3. (a) DFT-calculated band structure of the **graphene/MnPSe<sub>3</sub>** heterostructure along the high-symmetry path M-K- $\Gamma$  without SOC, when the MnPSe<sub>3</sub> is in the **antiferromagnetic zigzag phase**. Red solid (blue dashed) lines correspond to spin up (spin down). (b) Zoom to the DFT-calculated (symbols) low energy Dirac bands near the K point with a fit to the model Hamiltonian (solid line). (c) The splitting of valence and conduction band.

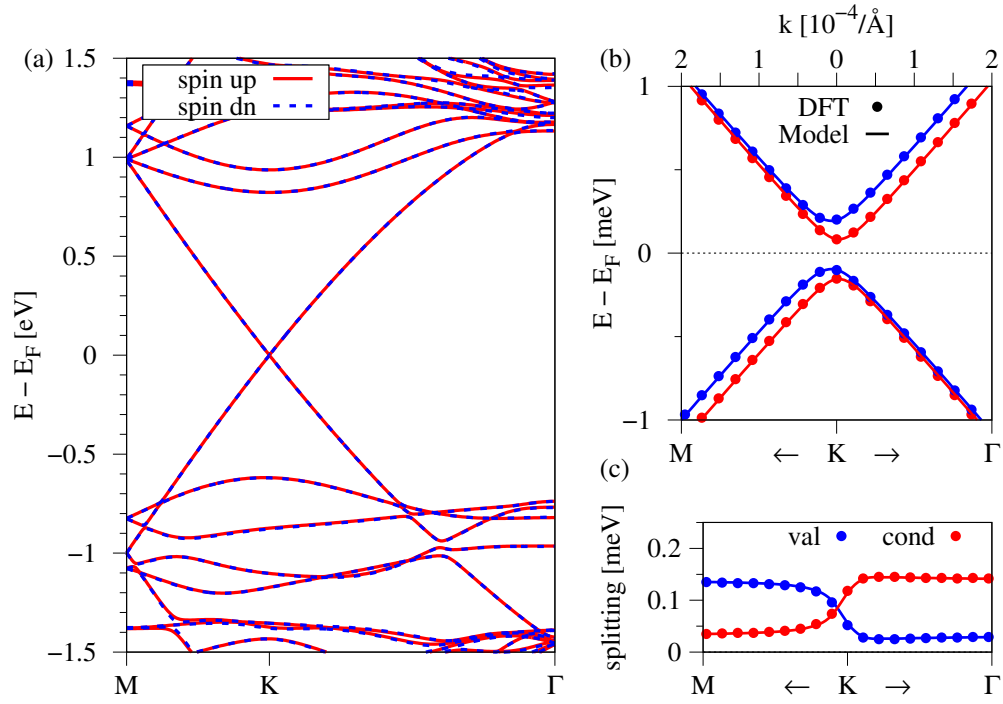

FIG. S4. (a) DFT-calculated band structure of the **graphene/MnPSe<sub>3</sub>** heterostructure along the high-symmetry path M-K- $\Gamma$  without SOC, when the MnPSe<sub>3</sub> is in the **antiferromagnetic stripy phase**. Red solid (blue dashed) lines correspond to spin up (spin down). (b) Zoom to the DFT-calculated (symbols) low energy Dirac bands near the K point with a fit to the model Hamiltonian (solid line). (c) The splitting of valence and conduction band.

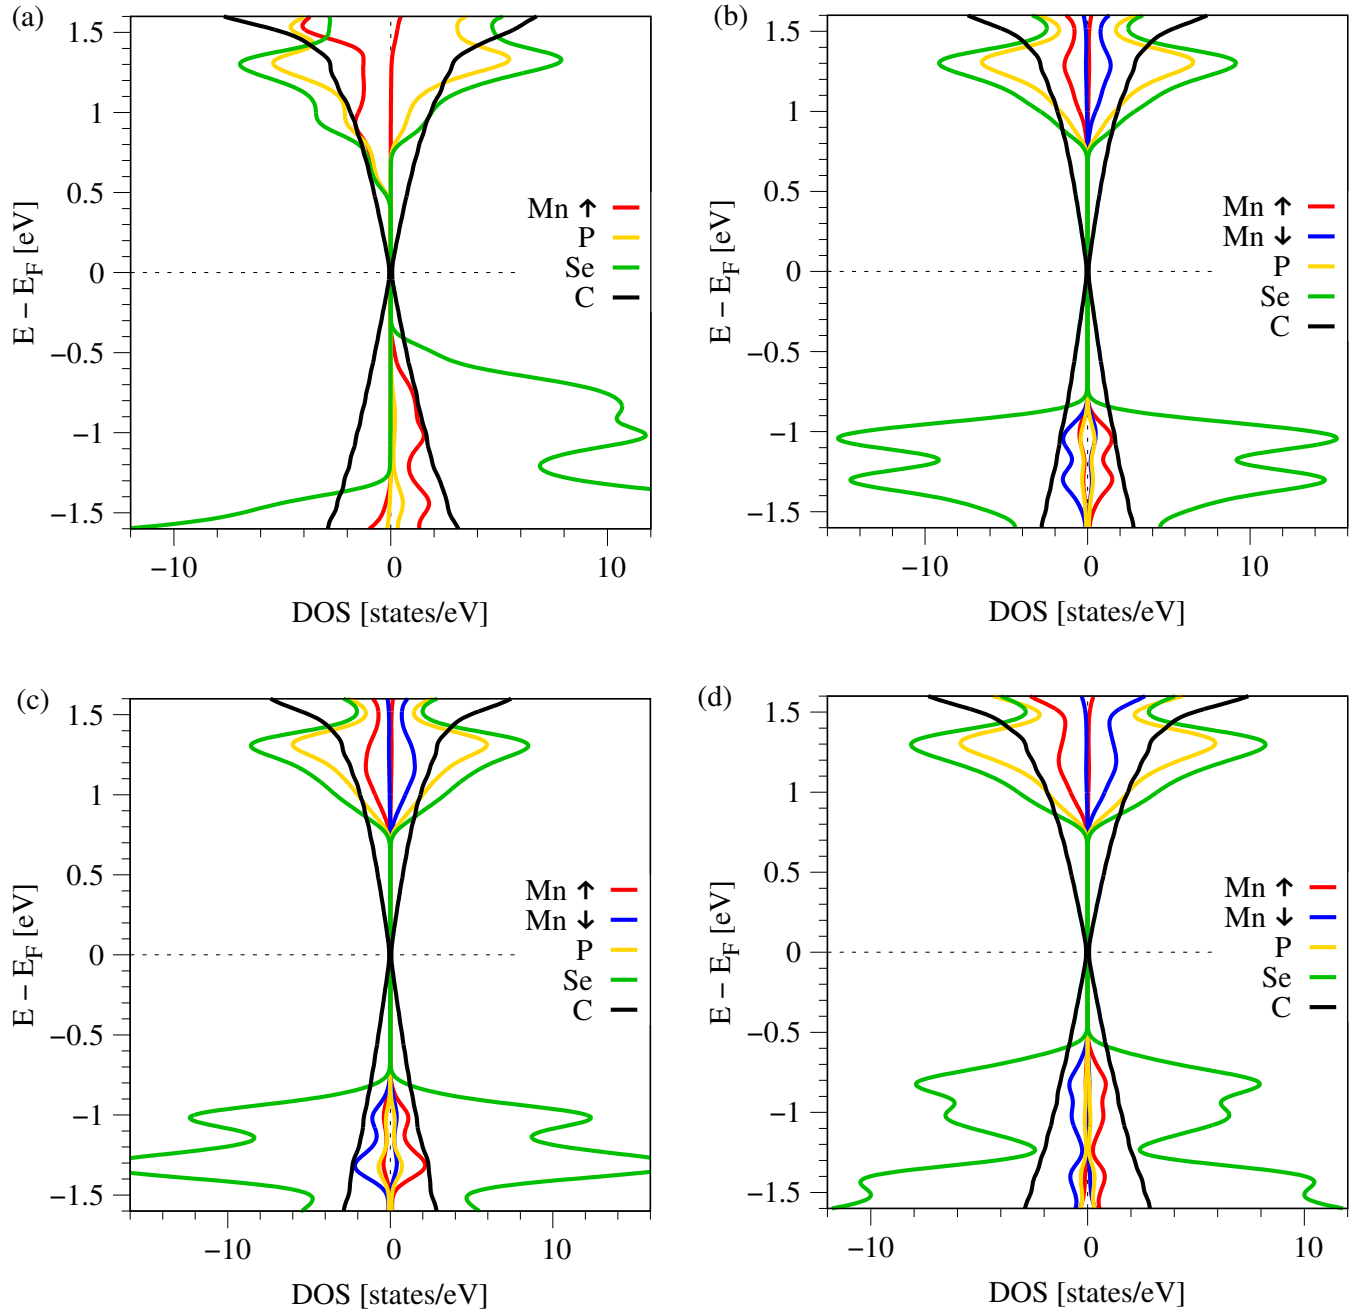

FIG. S5. Spin and atom resolved Density of States (DOS) for graphene on MnPSe<sub>3</sub> when MnPSe<sub>3</sub> is in the (a) ferromagnetic, (b) antiferromagnetic Néel, (c) antiferromagnetic zigzag, or (d) antiferromagnetic stripy phase.

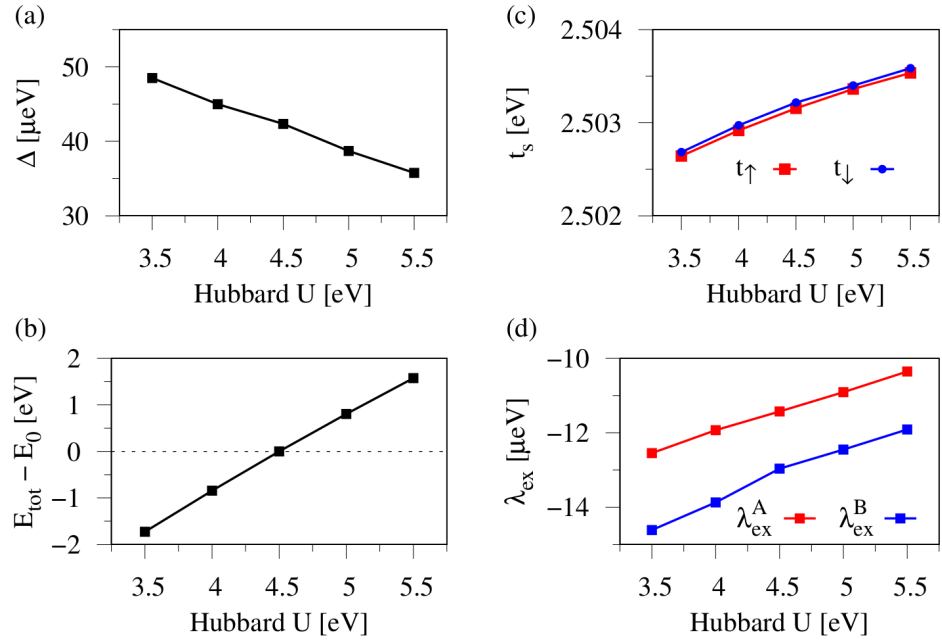

FIG. S6. Hubbard  $U$  dependence of (a) the staggered potential  $\Delta$ , (b) the total energy  $E_{\text{tot}}$ , (c) the spin dependent hopping parameters  $t_{\uparrow}$  and  $t_{\downarrow}$ , and (d) the sublattice resolved proximity exchange parameters  $\lambda_{\text{ex}}^A$  and  $\lambda_{\text{ex}}^B$  for the **graphene/MnPSe<sub>3</sub>** heterostructure when the MnPSe<sub>3</sub> is in the **antiferromagnetic Néel phase**.

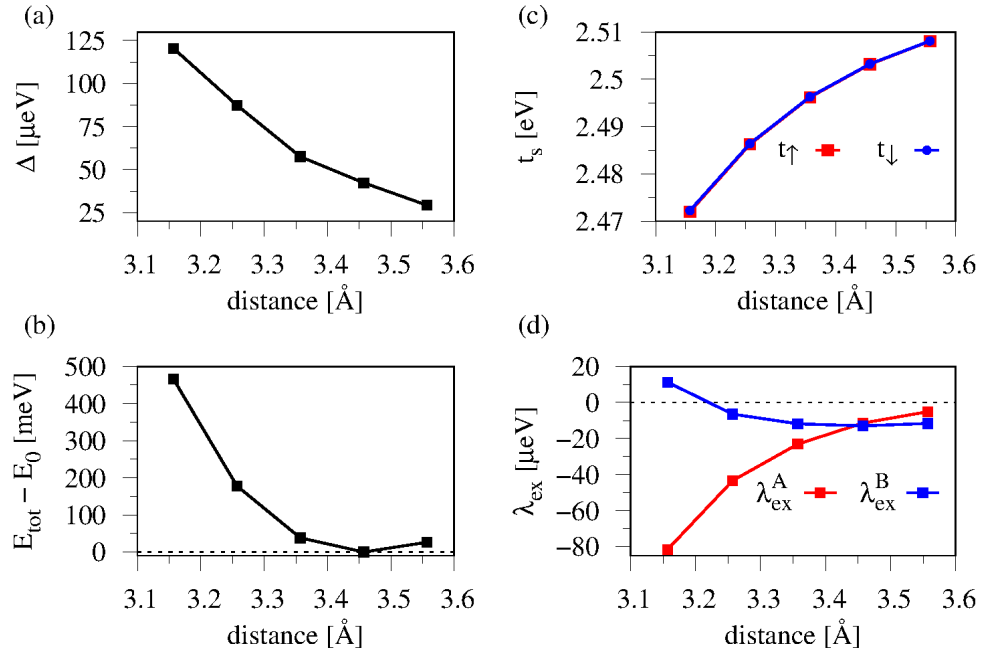

FIG. S7. Interlayer distance dependence of (a) the staggered potential  $\Delta$ , (b) the total energy  $E_{\text{tot}}$ , (c) the spin dependent hopping parameters  $t_{\uparrow}$  and  $t_{\downarrow}$ , and (d) the sublattice resolved proximity exchange parameters  $\lambda_{\text{ex}}^A$  and  $\lambda_{\text{ex}}^B$  for the **graphene/MnPSe<sub>3</sub>** heterostructure when the MnPSe<sub>3</sub> is in the **antiferromagnetic Néel phase**.

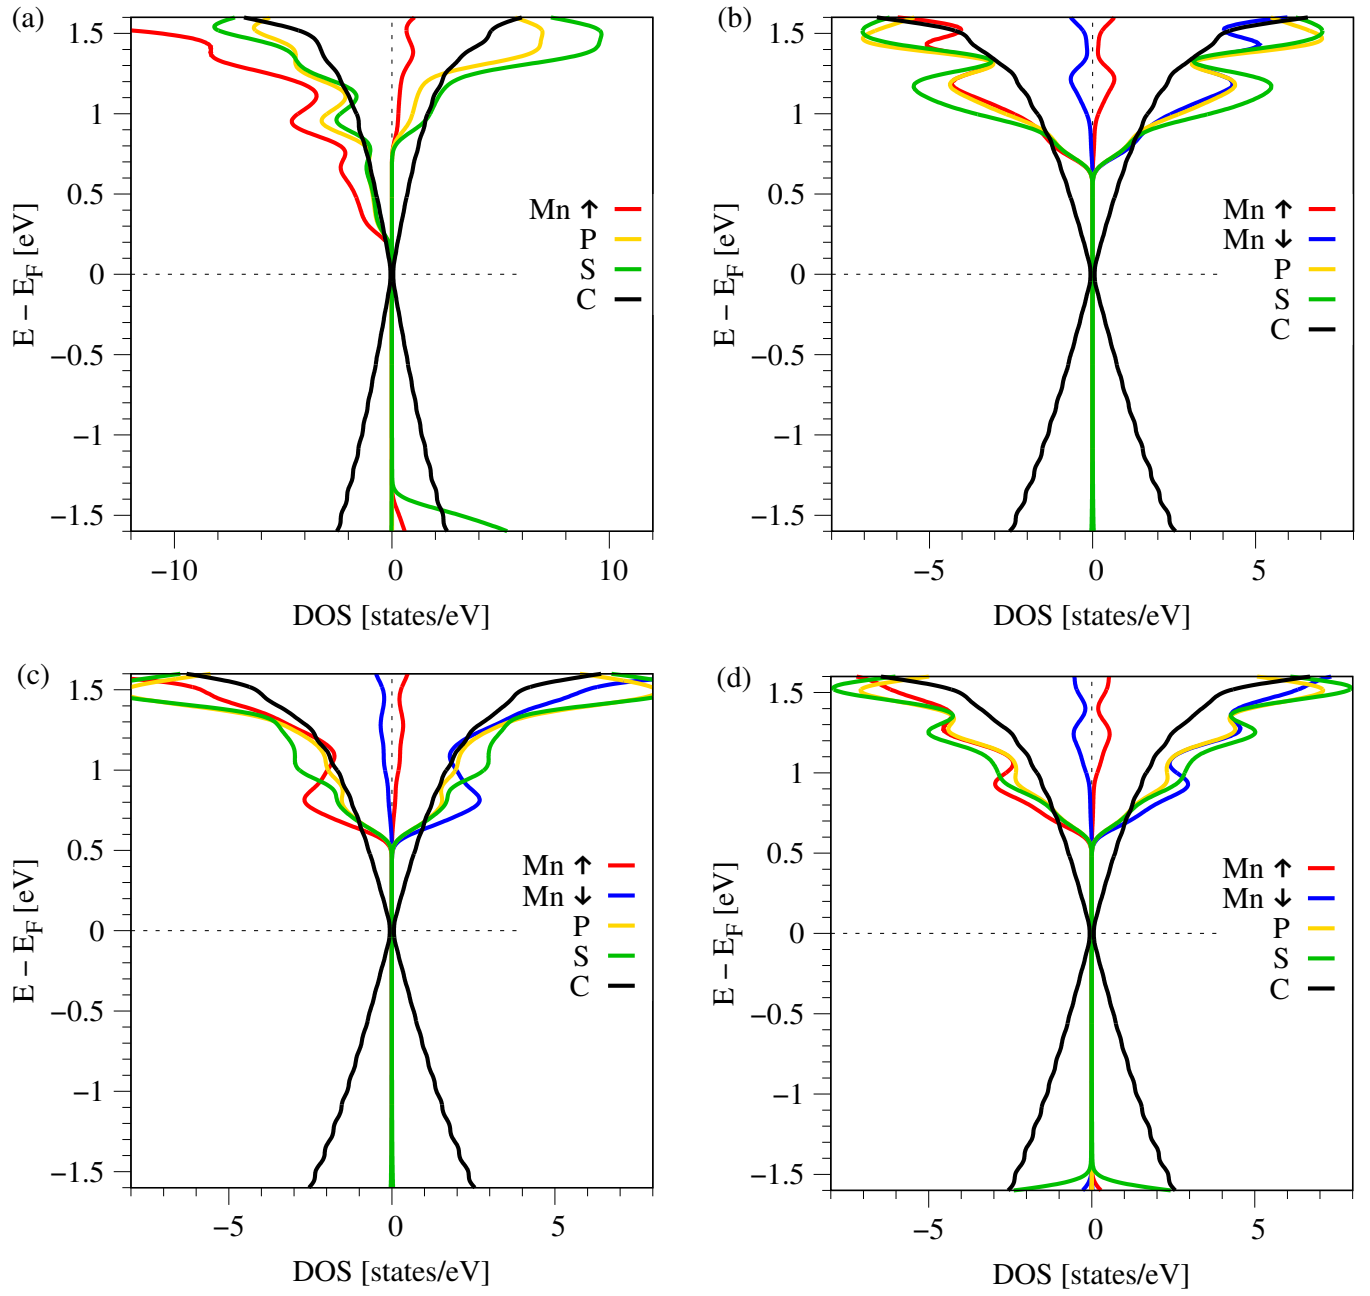

FIG. S8. Spin and atom resolved Density of States (DOS) for graphene on MnPS<sub>3</sub> when MnPS<sub>3</sub> is in the (a) ferromagnetic, (b) antiferromagnetic Néel, (c) antiferromagnetic zigzag, or (d) antiferromagnetic stripy phase.

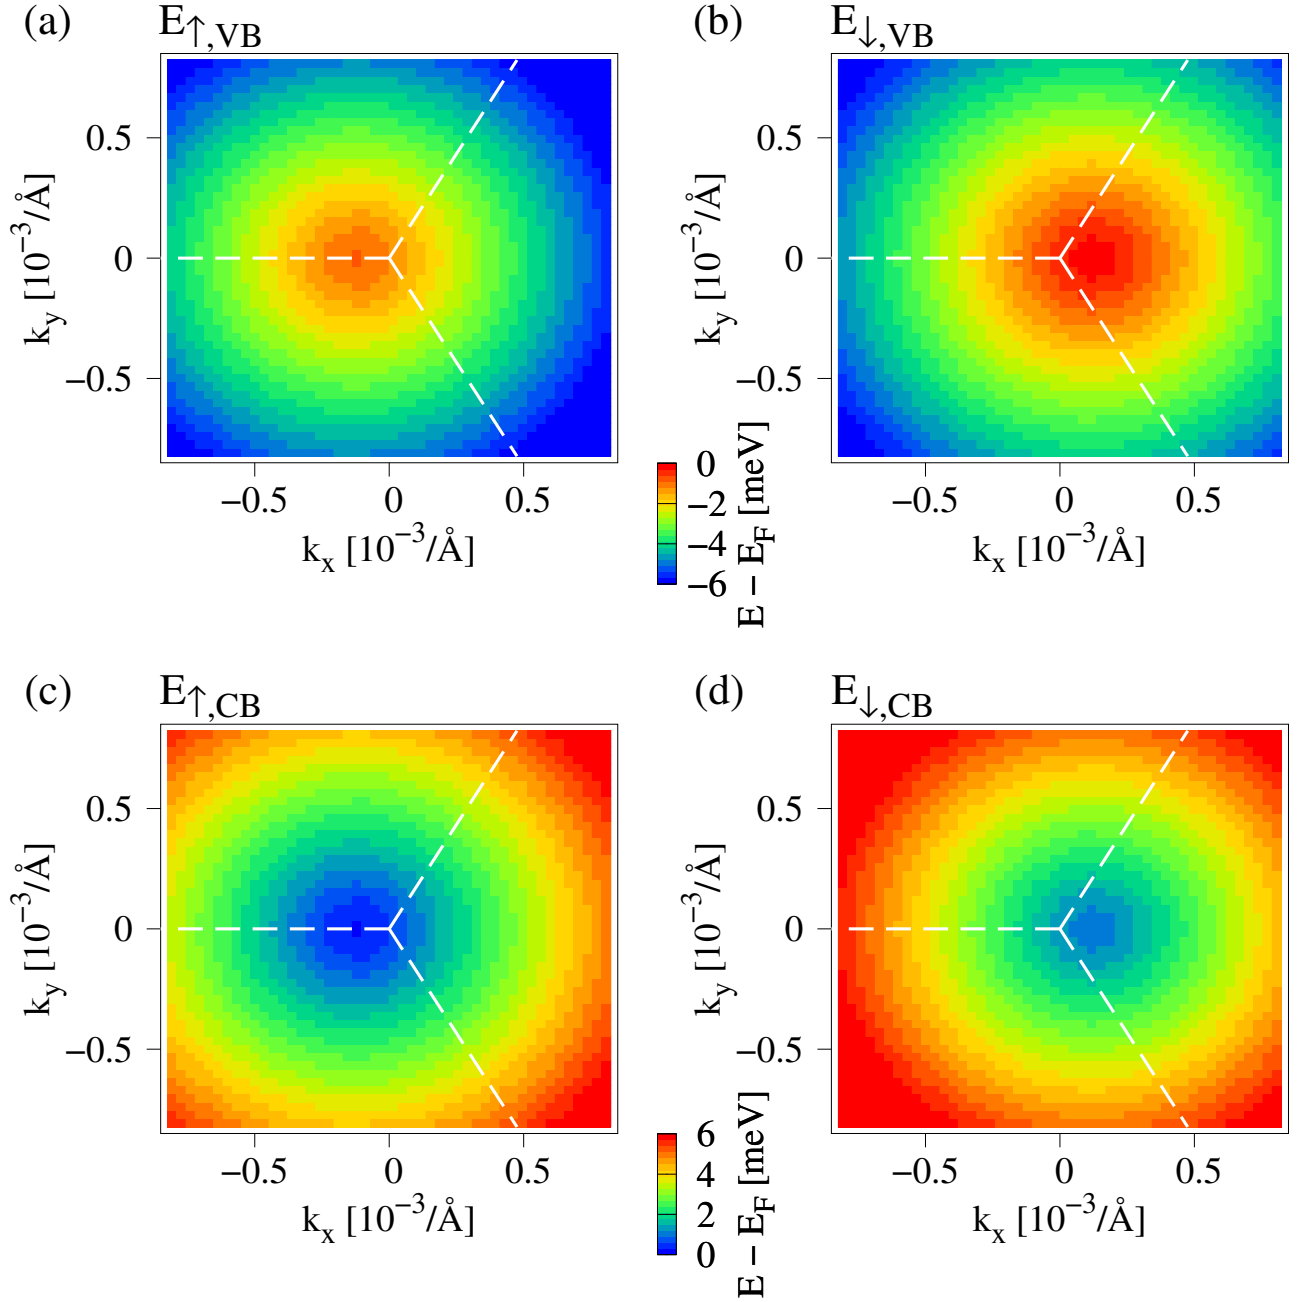

FIG. S9. 2D-map of the DFT-calculated low energy Dirac bands of the **graphene/MnPS<sub>3</sub>** heterostructure without SOC, when the MnPS<sub>3</sub> is in the **antiferromagnetic zigzag phase**. (a,b) The valence band energies for spin up  $E_{\uparrow,VB}$  and down  $E_{\downarrow,VB}$ . (c,d) Same as (a,b) but for the conduction band. The dashed white lines mark the edges of the Brillouin zone with the K point at the center.

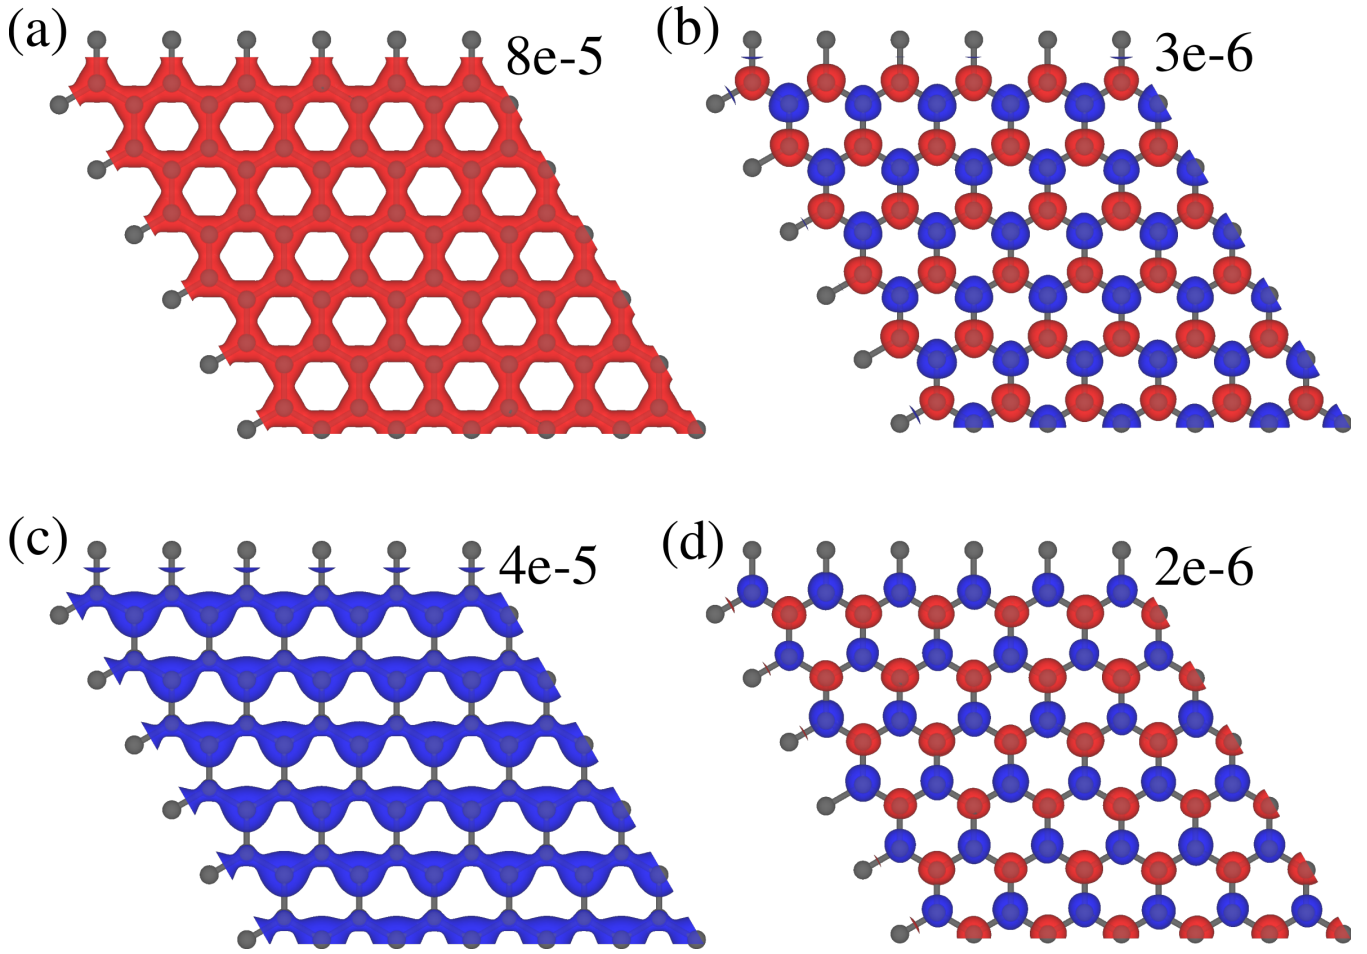

FIG. S10. Calculated spin polarizations,  $\Delta\rho = \rho_{\uparrow} - \rho_{\downarrow}$ , for **graphene on MnPS<sub>3</sub>** when MnPS<sub>3</sub> is in the (a) ferromagnetic, (b) antiferromagnetic Néel, (c) antiferromagnetic zigzag, or (d) antiferromagnetic stripy phase. For better visualization of the spin polarizations on graphene, we have deleted the MnPS<sub>3</sub> substrate in the figures. The spin densities  $\rho_{\uparrow/\downarrow}(\mathbf{r}) = \sum_{n,\mathbf{k}} |\phi_{n,\uparrow/\downarrow}^{\mathbf{k}}(\mathbf{r})|^2$  are sums over eigenstates with the corresponding spin. Here, we take into account Dirac states in the energy window of  $-6$  to  $-4$  meV below the Fermi level. The color red (blue) corresponds to  $\Delta\rho > 0$  ( $\Delta\rho < 0$ ). The isosurfaces correspond to isovalues, in units  $\text{\AA}^{-3}$ , as indicated next to each subfigure.



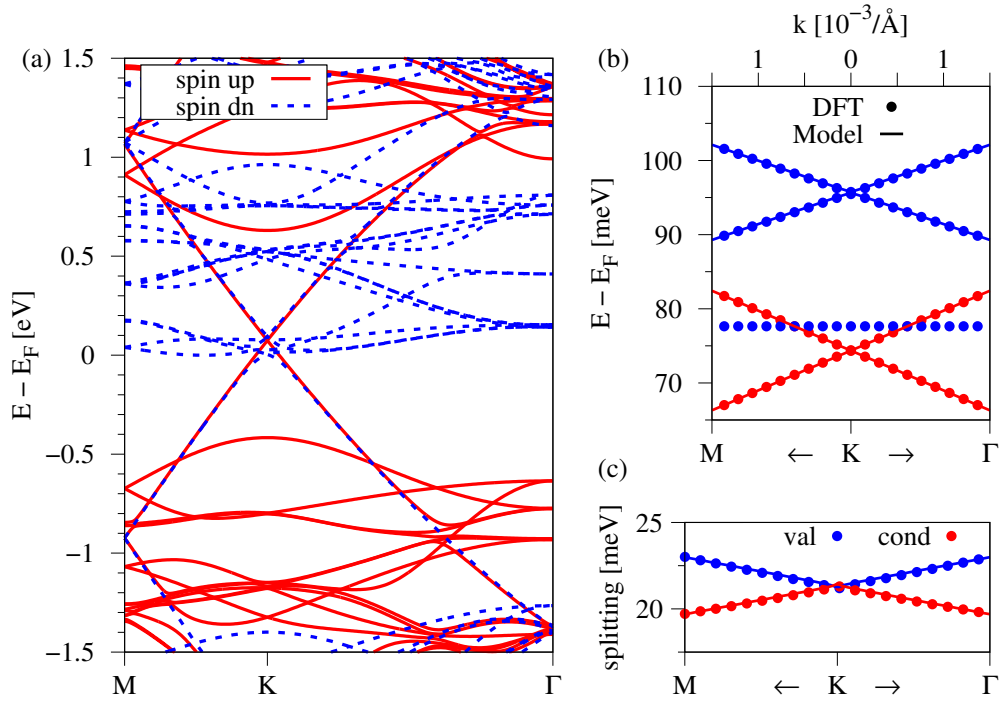

FIG. S11. (a) DFT-calculated band structure of the **graphene/NiPSe<sub>3</sub>** heterostructure along the high-symmetry path M-K- $\Gamma$  without SOC, when the NiPSe<sub>3</sub> is in the **ferromagnetic phase**. Red solid (blue dashed) lines correspond to spin up (spin down). (b) Zoom to the DFT-calculated (symbols) low energy Dirac bands near the K point with a fit to the model Hamiltonian (solid line). (c) The splitting of valence and conduction band.

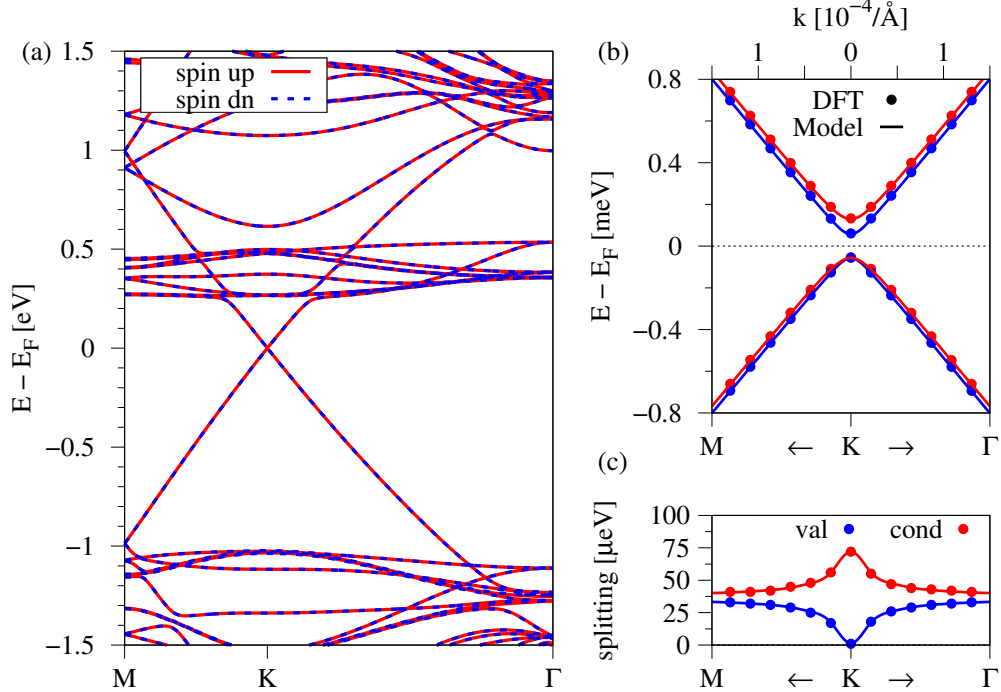

FIG. S12. (a) DFT-calculated band structure of the **graphene/NiPSe<sub>3</sub>** heterostructure along the high-symmetry path M-K- $\Gamma$  without SOC, when the NiPSe<sub>3</sub> is in the **antiferromagnetic Néel phase**. Red solid (blue dashed) lines correspond to spin up (spin down). (b) Zoom to the DFT-calculated (symbols) low energy Dirac bands near the K point with a fit to the model Hamiltonian (solid line). (c) The splitting of valence and conduction band.

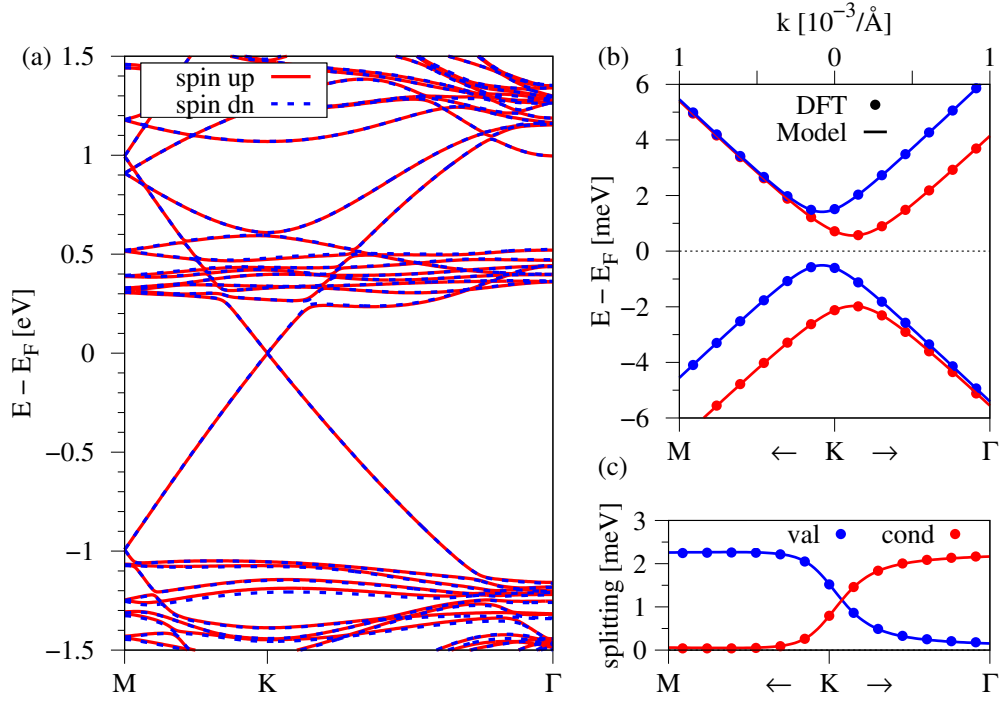

FIG. S13. (a) DFT-calculated band structure of the **graphene/NiPSe<sub>3</sub>** heterostructure along the high-symmetry path M-K- $\Gamma$  without SOC, when the NiPSe<sub>3</sub> is in the **antiferromagnetic zigzag phase**. Red solid (blue dashed) lines correspond to spin up (spin down). (b) Zoom to the DFT-calculated (symbols) low energy Dirac bands near the K point with a fit to the model Hamiltonian (solid line). (c) The splitting of valence and conduction band.

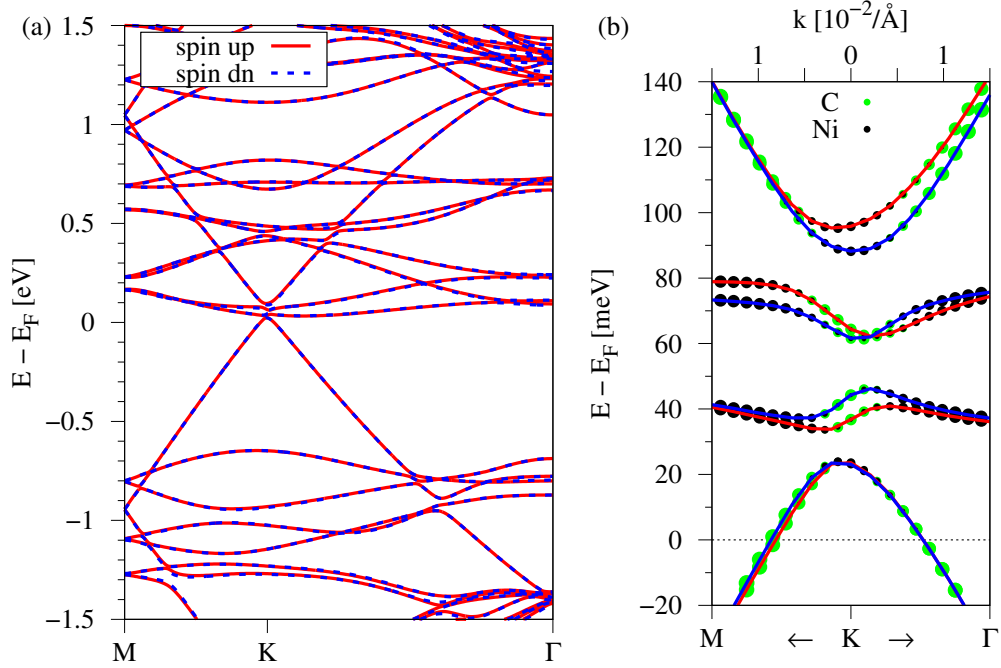

FIG. S14. (a) DFT-calculated band structure of the **graphene/NiPSe<sub>3</sub>** heterostructure along the high-symmetry path M-K- $\Gamma$  without SOC, when the NiPSe<sub>3</sub> is in the **antiferromagnetic stripy phase**. Red solid (blue dashed) lines correspond to spin up (spin down). (b) Zoom to the DFT-calculated low energy Dirac bands near the K point (red and blue solid lines for spin up and down). The green and black spheres represent the projections onto C and Ni states. This emphasizes that the graphene Dirac states are strongly hybridized with Ni states from the NiPSe<sub>3</sub> and we cannot apply our model fit properly.

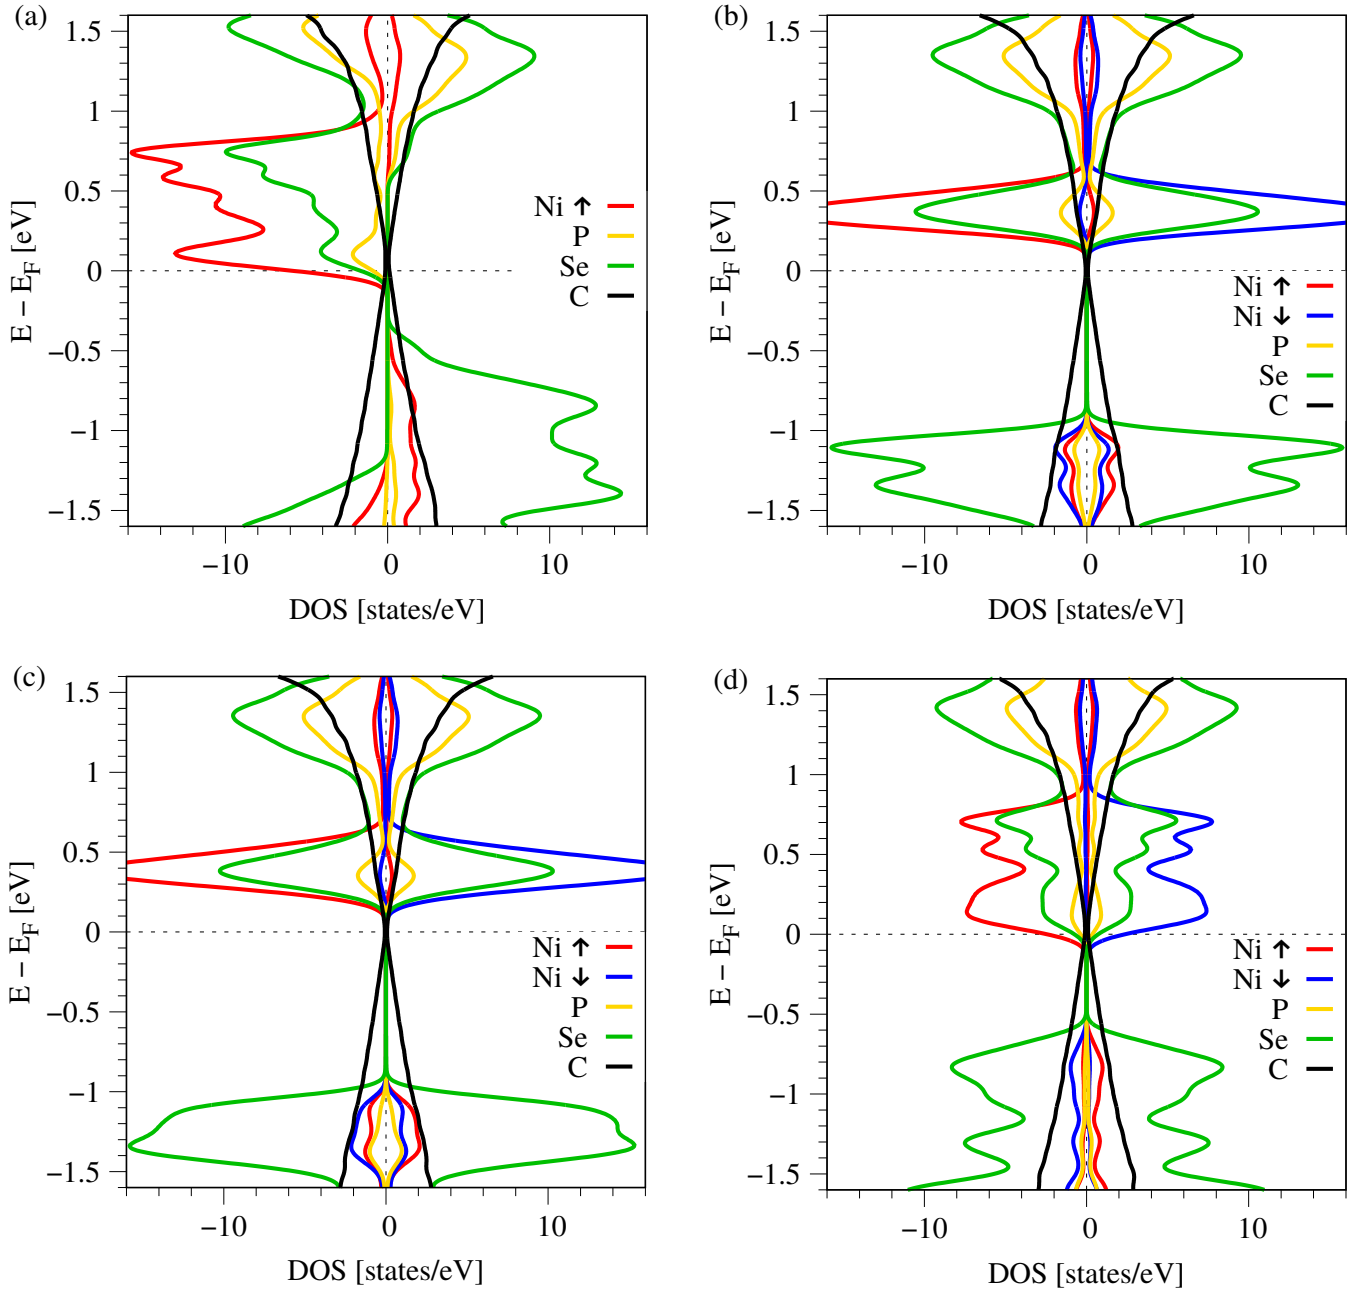

FIG. S15. Spin and atom resolved Density of States (DOS) for graphene on NiPSe<sub>3</sub> when NiPSe<sub>3</sub> is in the (a) ferromagnetic, (b) antiferromagnetic Néel, (c) antiferromagnetic zigzag, or (d) antiferromagnetic stripy phase.

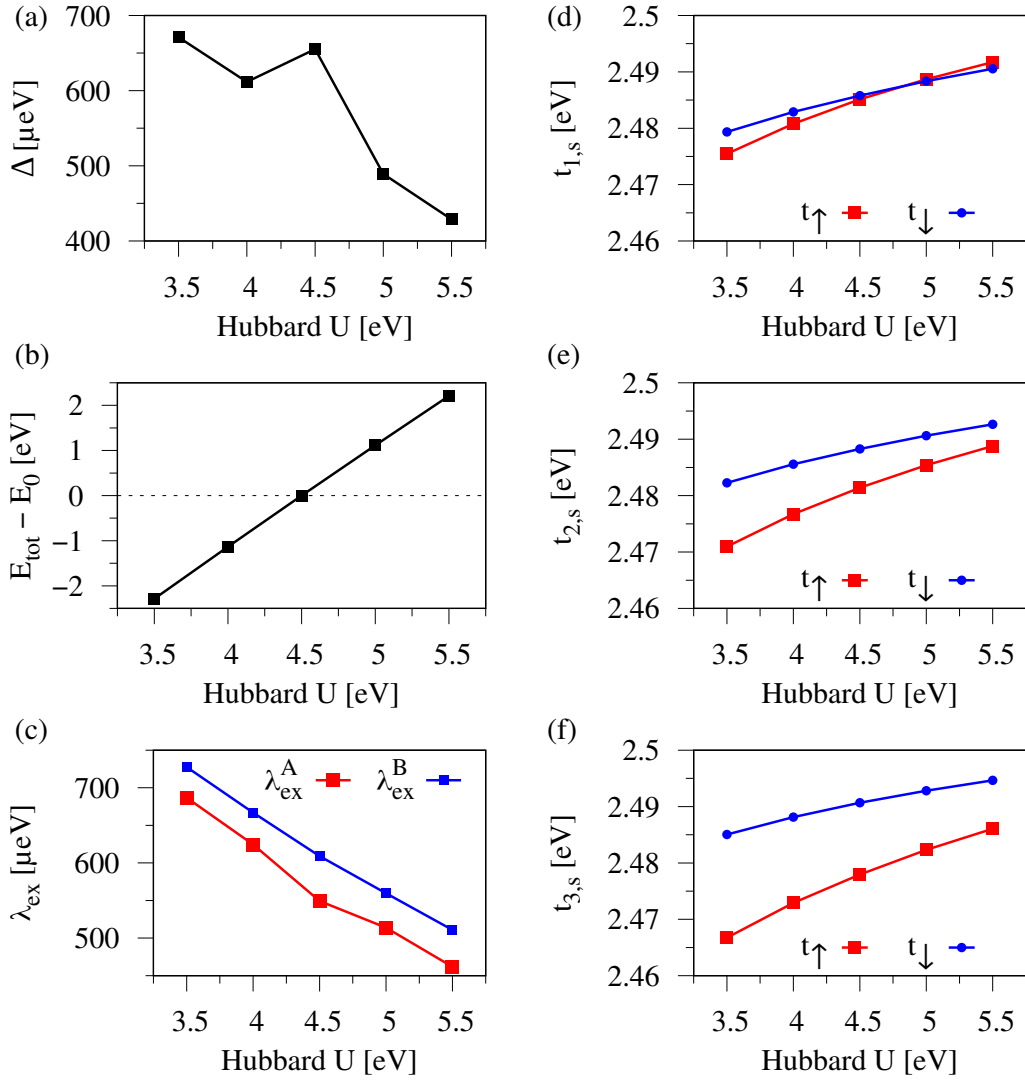

FIG. S16. Hubbard  $U$  dependence of (a) the staggered potential  $\Delta$ , (b) the total energy  $E_{\text{tot}}$ , (c) the sublattice resolved proximity exchange parameters  $\lambda_{\text{ex}}^A$  and  $\lambda_{\text{ex}}^B$ , and (d-f) the spin and direction dependent hopping parameters  $t_{\alpha,\uparrow}$  and  $t_{\alpha,\downarrow}$ , for the [graphene/NiPSe<sub>3</sub>](#) heterostructure when the NiPSe<sub>3</sub> is in the [antiferromagnetic zigzag](#) phase.

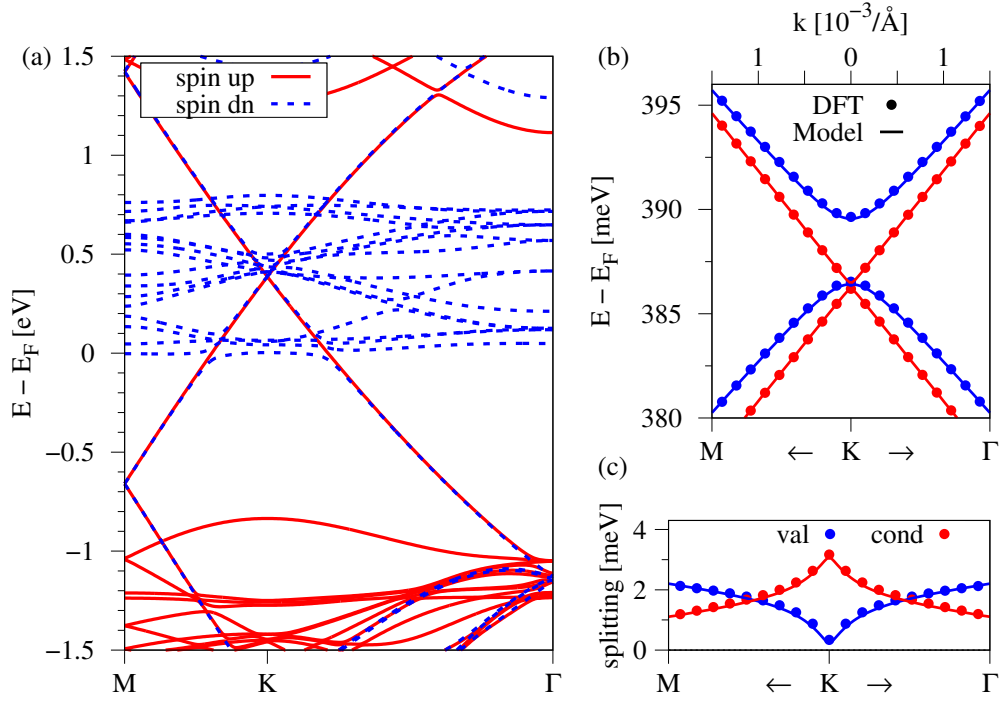

FIG. S17. (a) DFT-calculated band structure of the **graphene/NiPS<sub>3</sub>** heterostructure along the high-symmetry path M-K- $\Gamma$  without SOC, when the NiPS<sub>3</sub> is in the **ferromagnetic phase**. Red solid (blue dashed) lines correspond to spin up (spin down). (b) Zoom to the DFT-calculated (symbols) low energy Dirac bands near the K point with a fit to the model Hamiltonian (solid line). (c) The splitting of valence and conduction band.

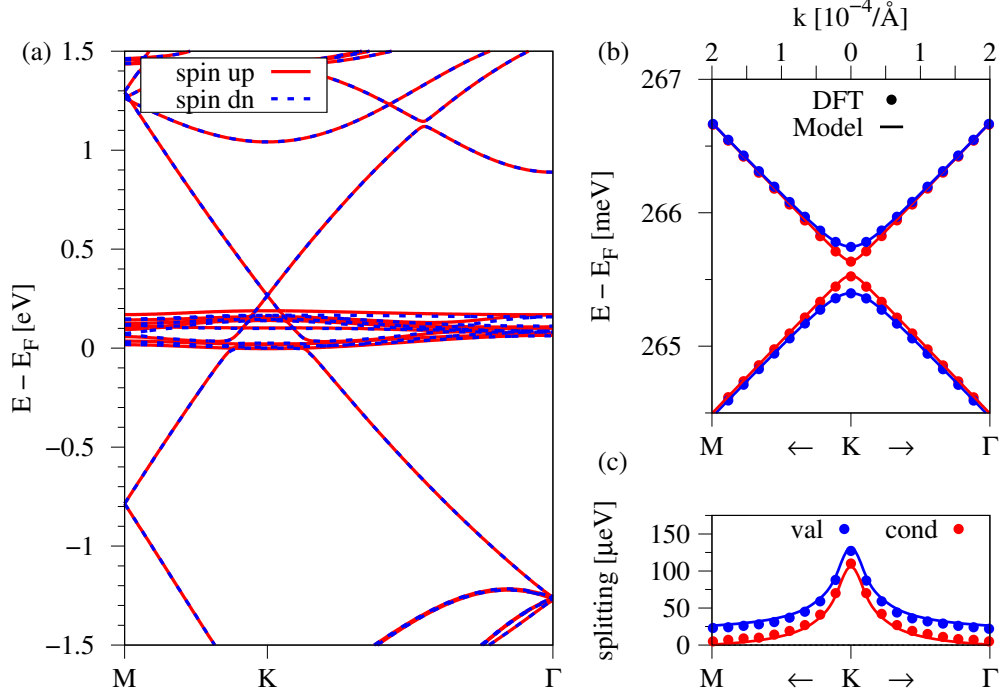

FIG. S18. (a) DFT-calculated band structure of the **graphene/NiPS<sub>3</sub>** heterostructure along the high-symmetry path M-K- $\Gamma$  without SOC, when the NiPS<sub>3</sub> is in the **antiferromagnetic Néel phase**. Red solid (blue dashed) lines correspond to spin up (spin down). (b) Zoom to the DFT-calculated (symbols) low energy Dirac bands near the K point with a fit to the model Hamiltonian (solid line). (c) The splitting of valence and conduction band.

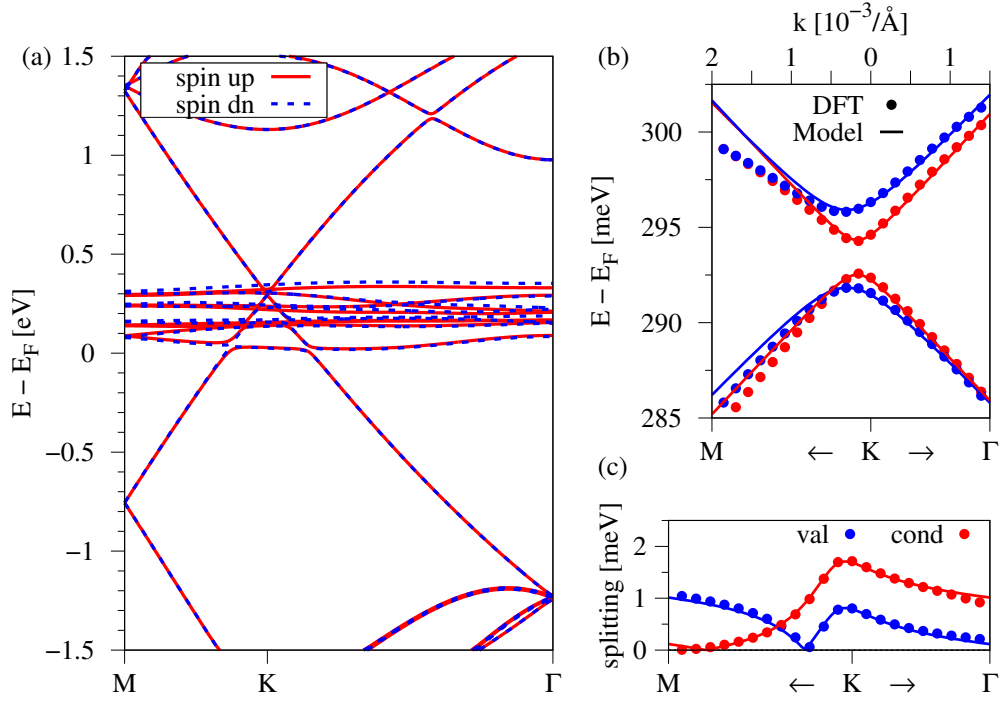

FIG. S19. (a) DFT-calculated band structure of the **graphene/NiPS<sub>3</sub>** heterostructure along the high-symmetry path M-K- $\Gamma$  without SOC, when the NiPS<sub>3</sub> is in the **antiferromagnetic zigzag phase**. Red solid (blue dashed) lines correspond to spin up (spin down). (b) Zoom to the DFT-calculated (symbols) low energy Dirac bands near the K point with a fit to the model Hamiltonian (solid line). (c) The splitting of valence and conduction band.

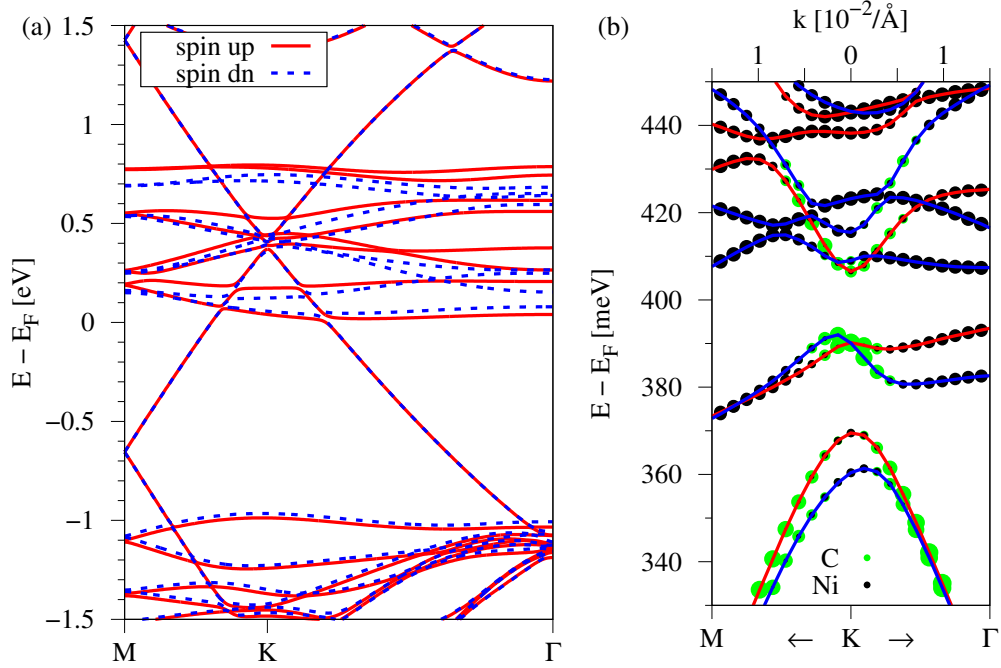

FIG. S20. (a) DFT-calculated band structure of the **graphene/NiPS<sub>3</sub>** heterostructure along the high-symmetry path M-K- $\Gamma$  without SOC, when the NiPS<sub>3</sub> is in the **antiferromagnetic stripy phase**. Red solid (blue dashed) lines correspond to spin up (spin down). (b) Zoom to the DFT-calculated low energy Dirac bands near the K point (red and blue solid lines for spin up and down). The green and black spheres represent the projections onto C and Ni states. This emphasizes that the graphene Dirac states are strongly hybridized with Ni states from the NiPS<sub>3</sub> and we cannot apply our model fit properly.

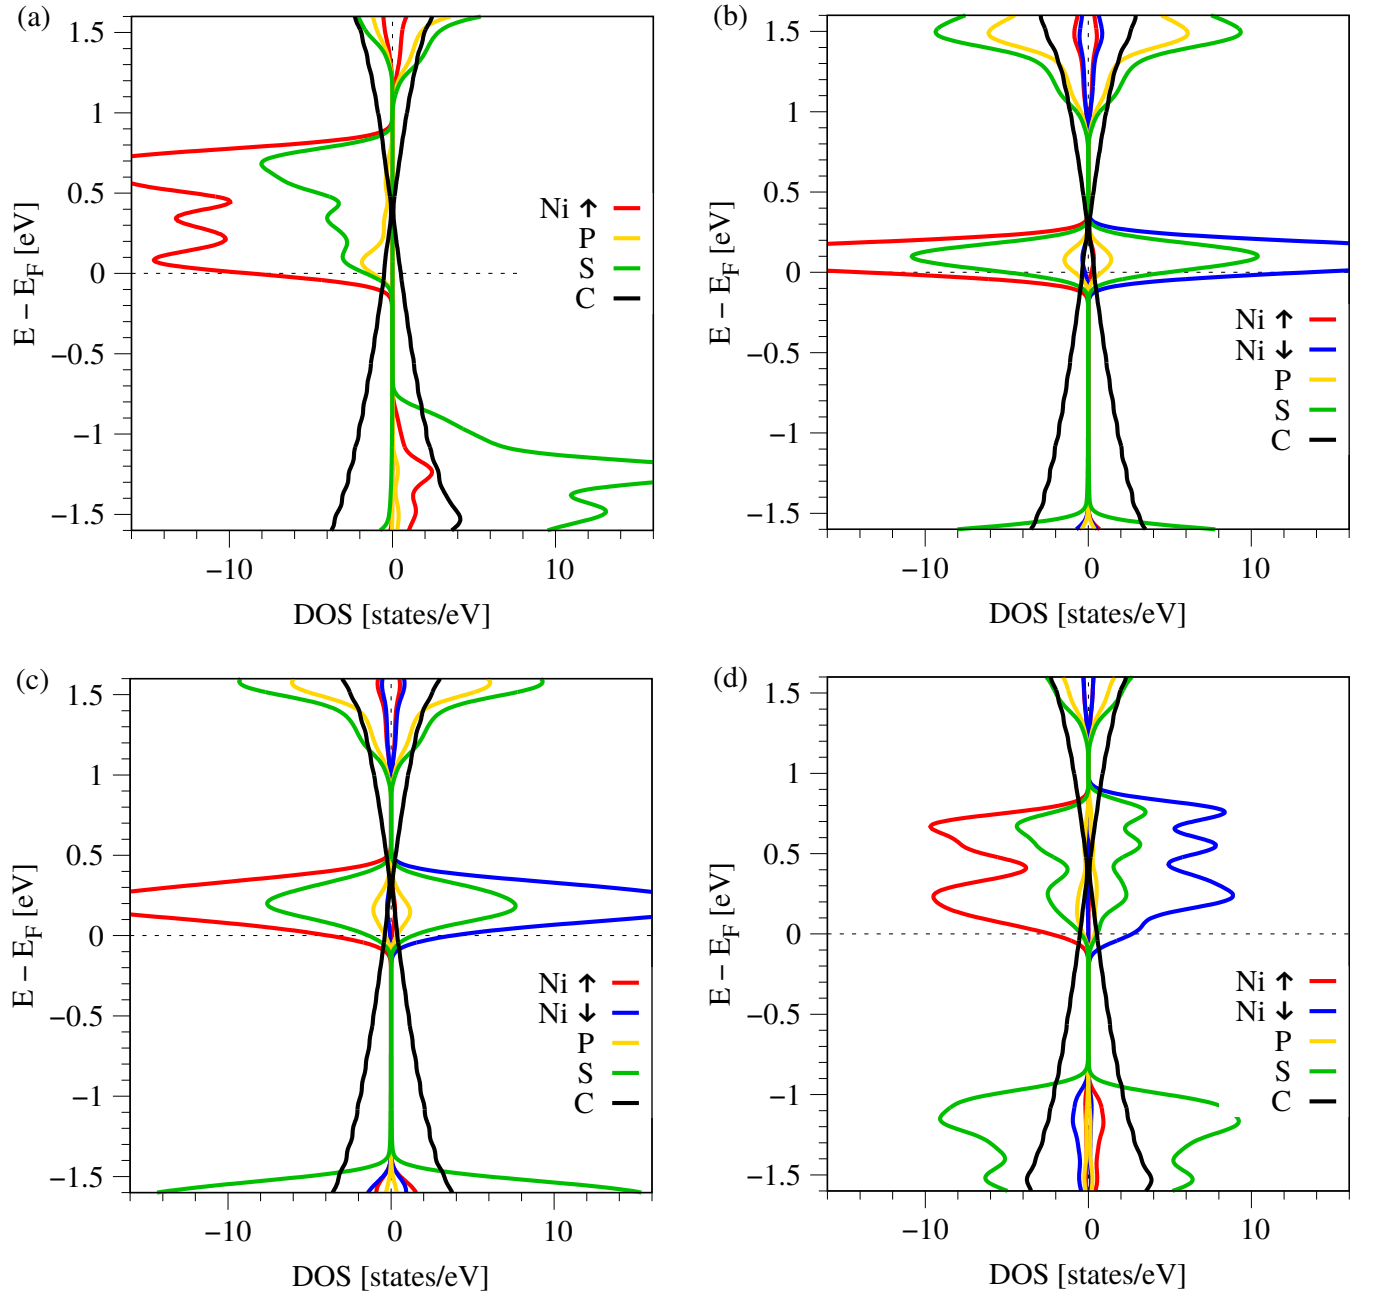

FIG. S21. Spin and atom resolved Density of States (DOS) for **graphene on  $\text{NiPS}_3$**  when  $\text{NiPS}_3$  is in the (a) ferromagnetic, (b) antiferromagnetic Néel, (c) antiferromagnetic zigzag, or (d) antiferromagnetic stripy phase.

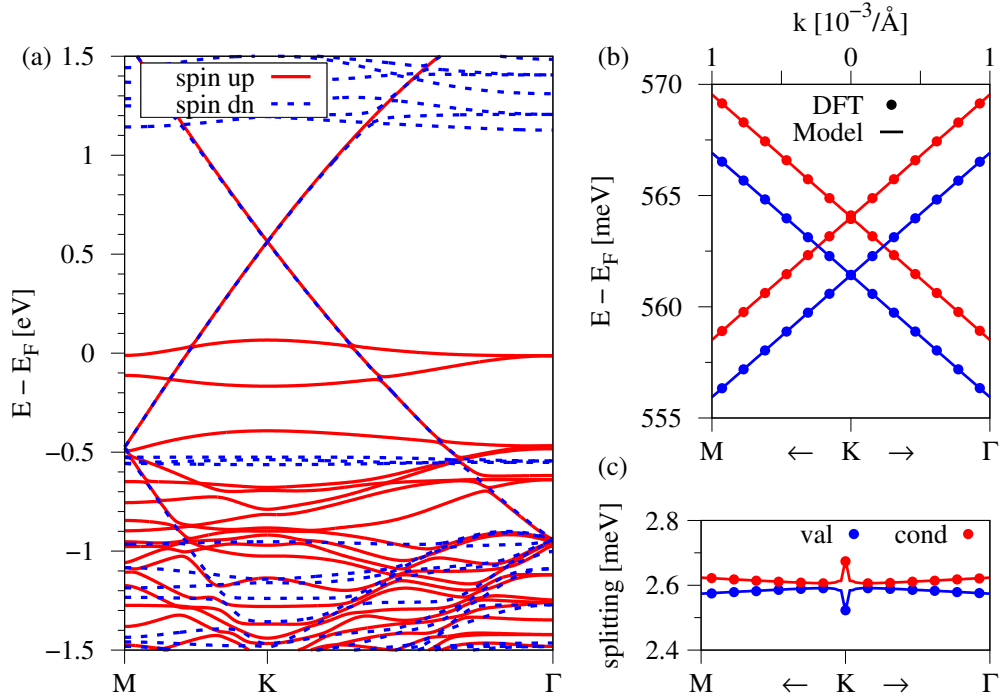

FIG. S22. (a) DFT-calculated band structure of the **graphene/CoPS<sub>3</sub>** heterostructure along the high-symmetry path M-K- $\Gamma$  without SOC, when the CoPS<sub>3</sub> is in the **ferromagnetic phase**. Red solid (blue dashed) lines correspond to spin up (spin down). (b) Zoom to the DFT-calculated (symbols) low energy Dirac bands near the K point with a fit to the model Hamiltonian (solid line). (c) The splitting of valence and conduction band.

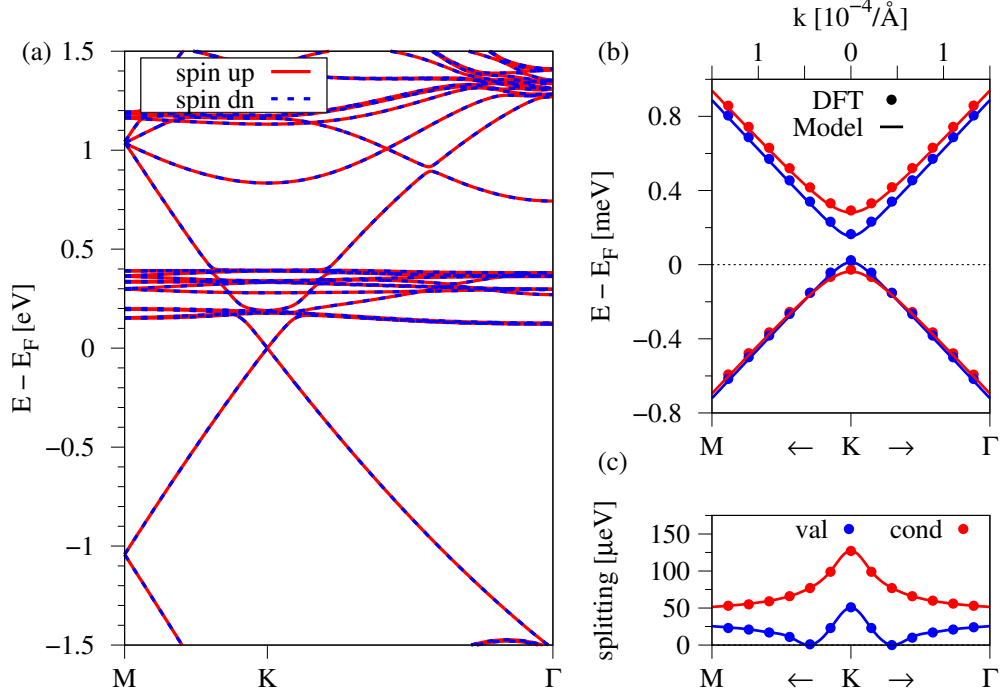

FIG. S23. (a) DFT-calculated band structure of the **graphene/CoPS<sub>3</sub>** heterostructure along the high-symmetry path M-K- $\Gamma$  without SOC, when the CoPS<sub>3</sub> is in the **antiferromagnetic Néel phase**. Red solid (spin down) (blue dashed) lines correspond to spin up (spin down). (b) Zoom to the DFT-calculated (symbols) low energy Dirac bands near the K point with a fit to the model Hamiltonian (solid line). (c) The splitting of valence and conduction band.



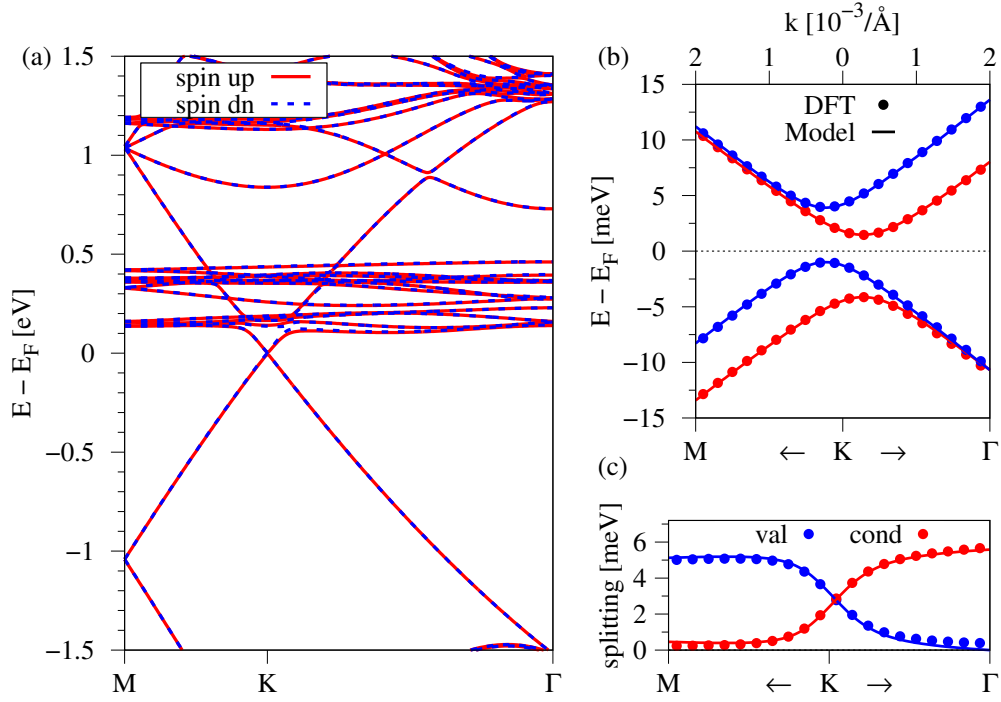

FIG. S24. (a) DFT-calculated band structure of the **graphene/CoPS<sub>3</sub>** heterostructure along the high-symmetry path M-K- $\Gamma$  without SOC, when the CoPS<sub>3</sub> is in the **antiferromagnetic zigzag phase**. Red solid (blue dashed) lines correspond to spin up (spin down). (b) Zoom to the DFT-calculated (symbols) low energy Dirac bands near the K point with a fit to the model Hamiltonian (solid line). (c) The splitting of valence and conduction band.

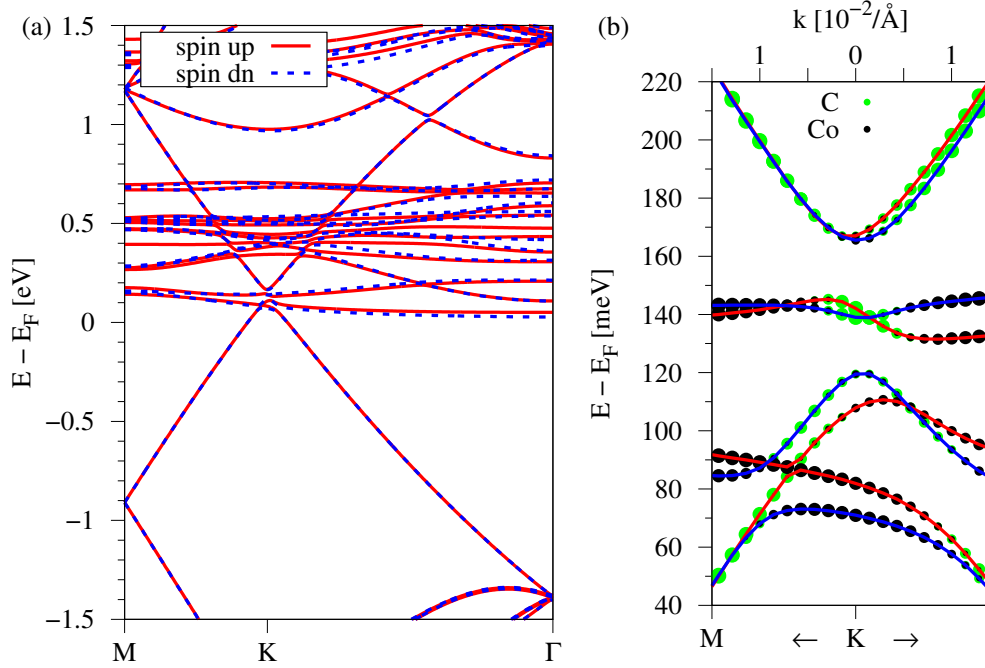

FIG. S25. (a) DFT-calculated band structure of the **graphene/CoPS<sub>3</sub>** heterostructure along the high-symmetry path M-K- $\Gamma$  without SOC, when the CoPS<sub>3</sub> is in the **antiferromagnetic stripy phase**. Red solid (blue dashed) lines correspond to spin up (spin down). (b) Zoom to the DFT-calculated low energy Dirac bands near the K point (red and blue solid lines for spin up and down). The green and black spheres represent the projections onto C and Co states. This emphasizes that the graphene Dirac states are strongly hybridized with Co states from the CoPS<sub>3</sub> and we cannot apply our model fit properly.

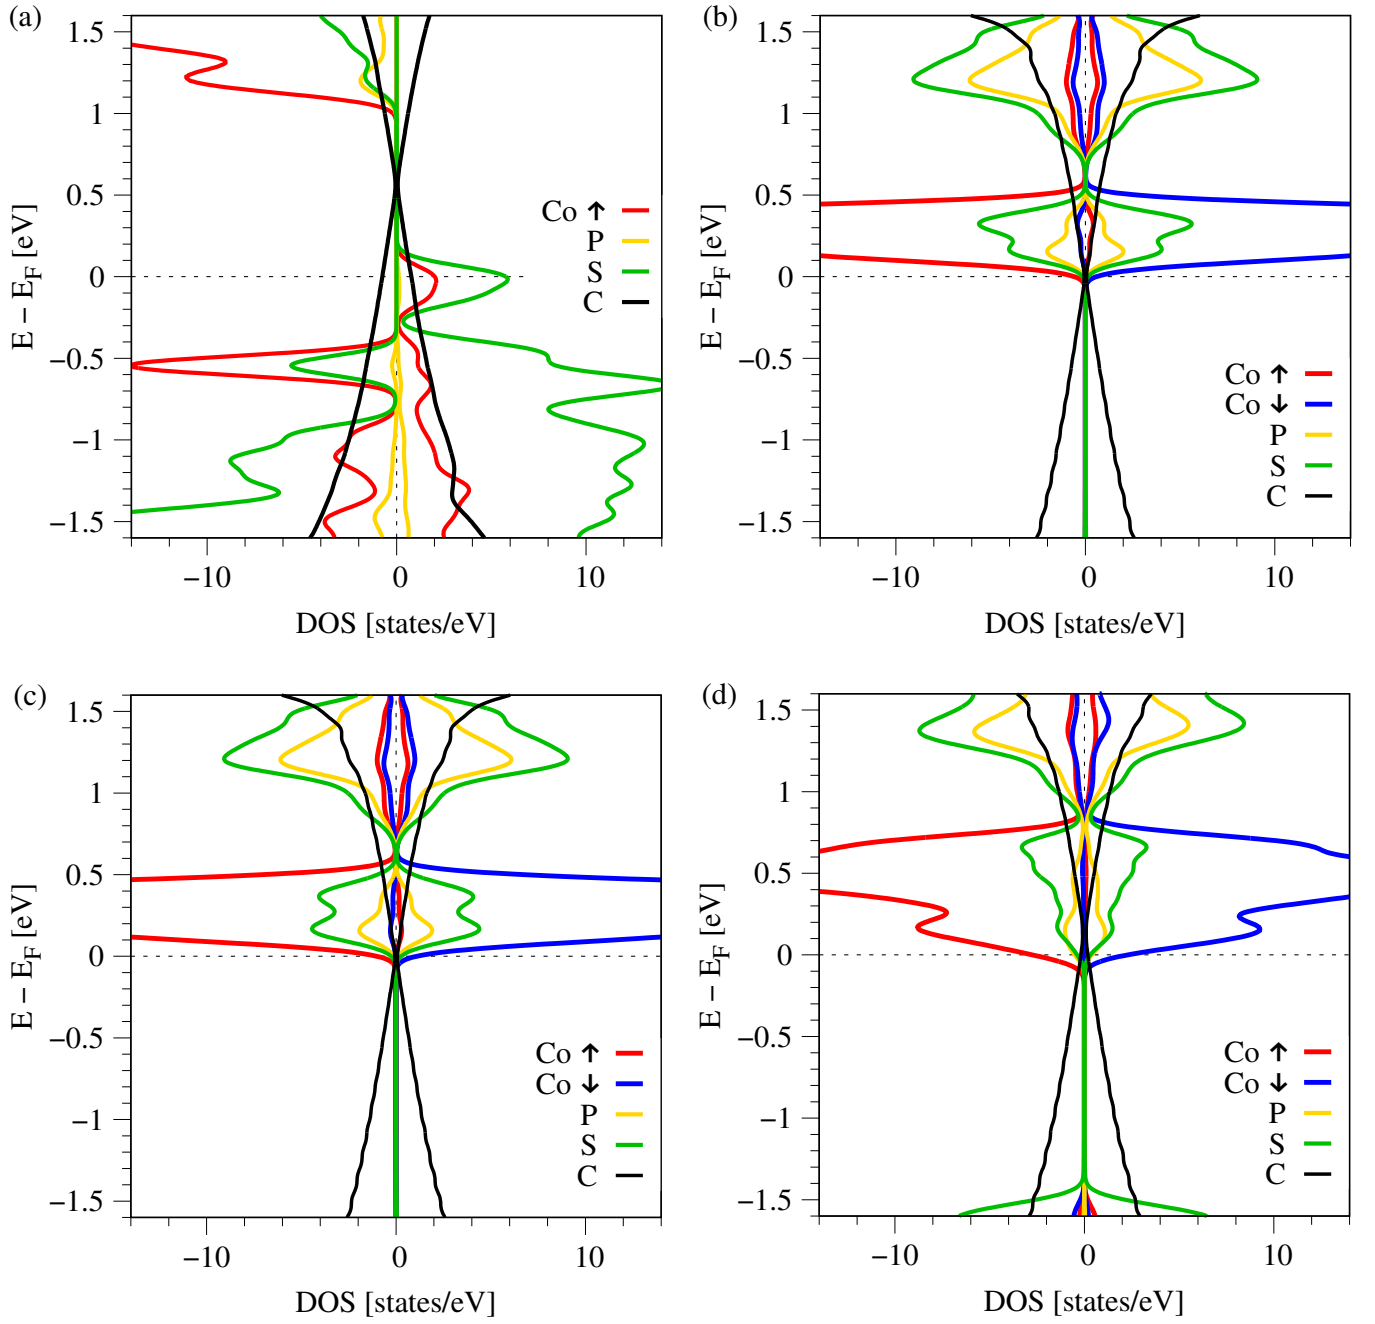

FIG. S26. Spin and atom resolved Density of States (DOS) for **graphene on CoPS<sub>3</sub>** when CoPS<sub>3</sub> is in the (a) ferromagnetic, (b) antiferromagnetic Néel, (c) antiferromagnetic zigzag, or (d) antiferromagnetic stripy phase.

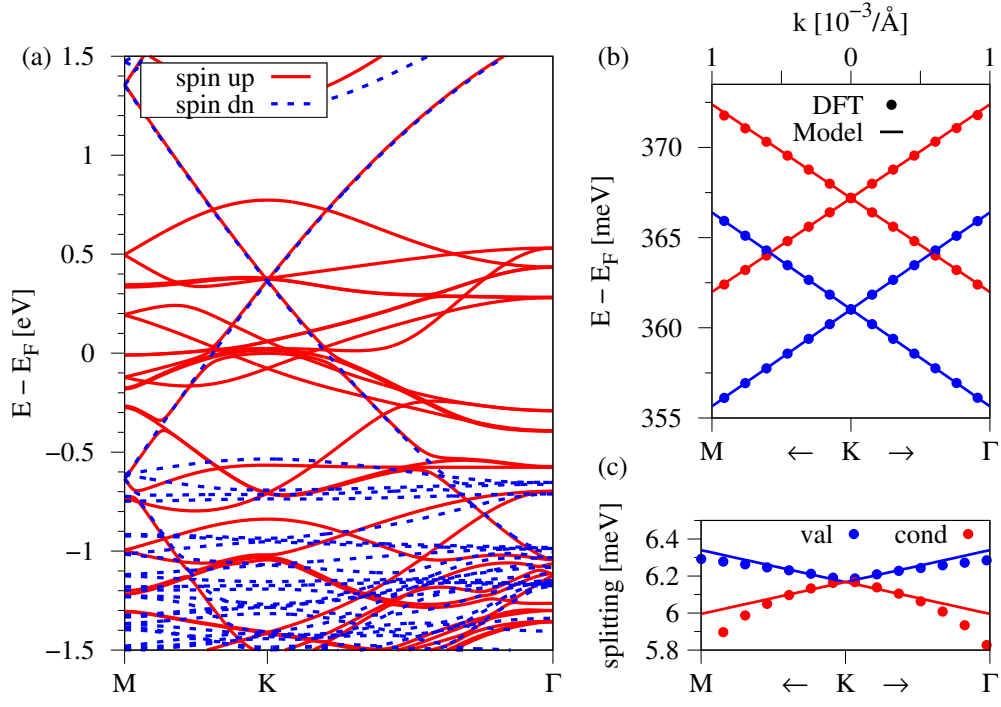

FIG. S27. (a) DFT-calculated band structure of the **graphene/CoPSe<sub>3</sub>** heterostructure along the high-symmetry path M-K- $\Gamma$  without SOC, when the CoPSe<sub>3</sub> is in the **ferromagnetic phase**. Red solid (blue dashed) lines correspond to spin up (spin down). (b) Zoom to the DFT-calculated (symbols) low energy Dirac bands near the K point with a fit to the model Hamiltonian (solid line). (c) The splitting of valence and conduction band.

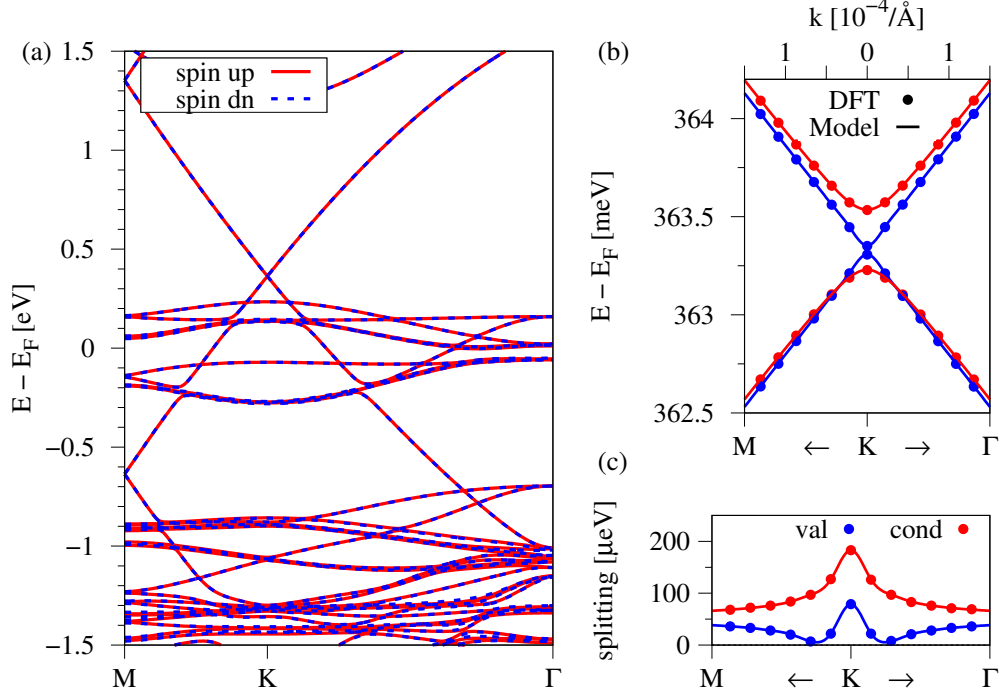

FIG. S28. (a) DFT-calculated band structure of the **graphene/CoPSe<sub>3</sub>** heterostructure along the high-symmetry path M-K- $\Gamma$  without SOC, when the CoPSe<sub>3</sub> is in the **antiferromagnetic Néel phase**. Red solid (blue dashed) lines correspond to spin up (spin down). (b) Zoom to the DFT-calculated (symbols) low energy Dirac bands near the K point with a fit to the model Hamiltonian (solid line). (c) The splitting of valence and conduction band.

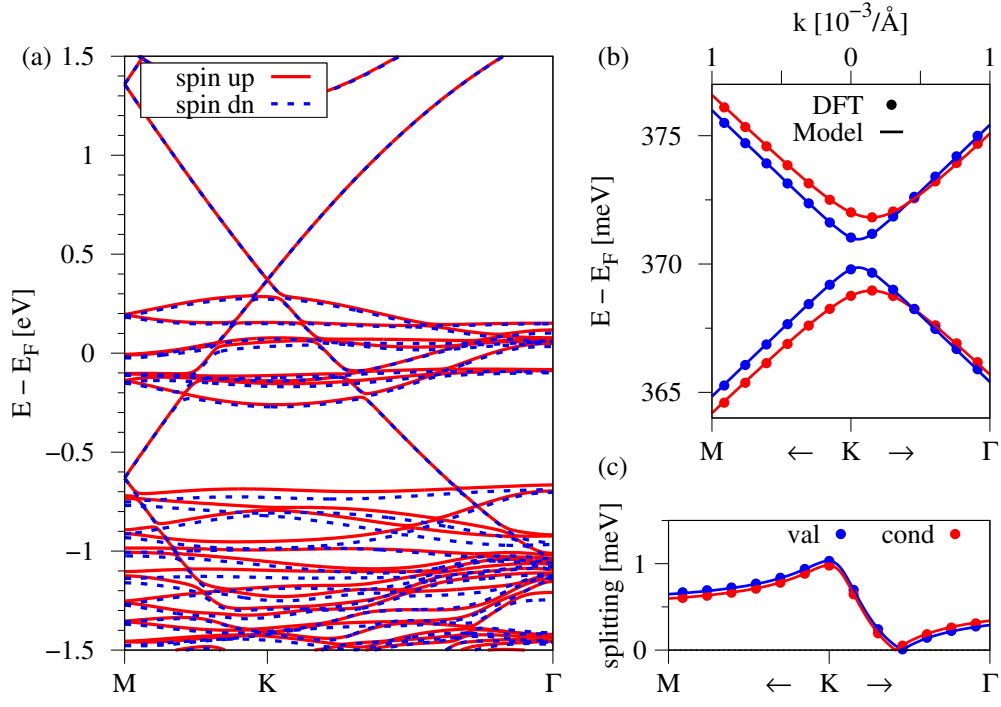

FIG. S29. (a) DFT-calculated band structure of the **graphene/CoPSe<sub>3</sub>** heterostructure along the high-symmetry path M-K- $\Gamma$  without SOC, when the CoPSe<sub>3</sub> is in the **antiferromagnetic zigzag phase**. Red solid (blue dashed) lines correspond to spin up (spin down). (b) Zoom to the DFT-calculated (symbols) low energy Dirac bands near the K point with a fit to the model Hamiltonian (solid line). (c) The splitting of valence and conduction band.

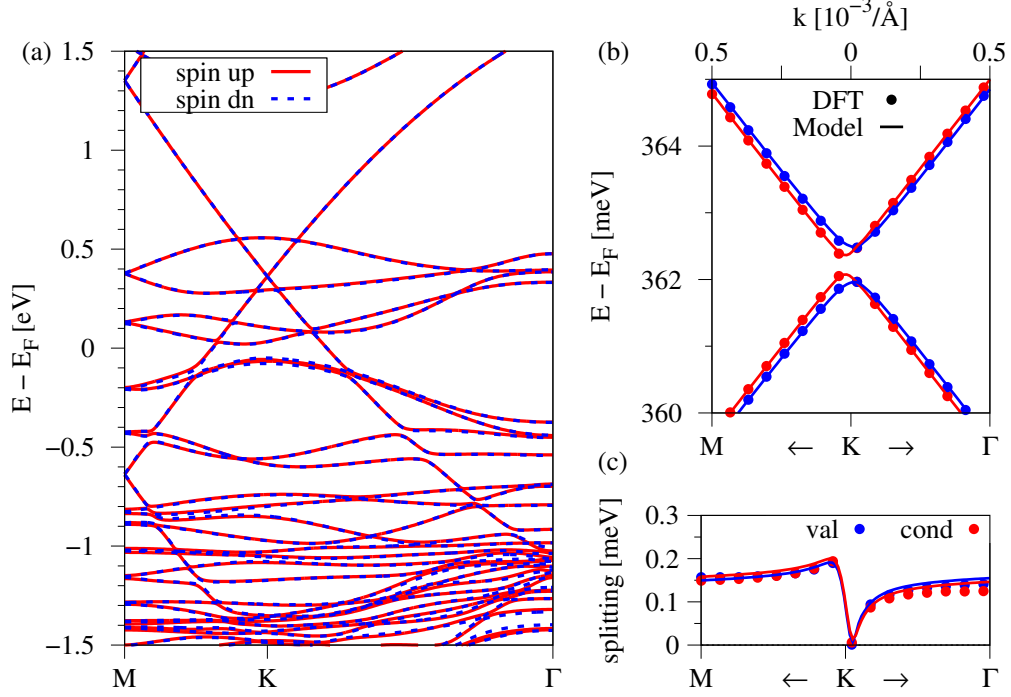

FIG. S30. (a) DFT-calculated band structure of the **graphene/CoPSe<sub>3</sub>** heterostructure along the high-symmetry path M-K- $\Gamma$  without SOC, when the CoPSe<sub>3</sub> is in the **antiferromagnetic stripy phase**. Red solid (blue dashed) lines correspond to spin up (spin down). (b) Zoom to the DFT-calculated (symbols) low energy Dirac bands near the K point with a fit to the model Hamiltonian (solid line). (c) The splitting of valence and conduction band.

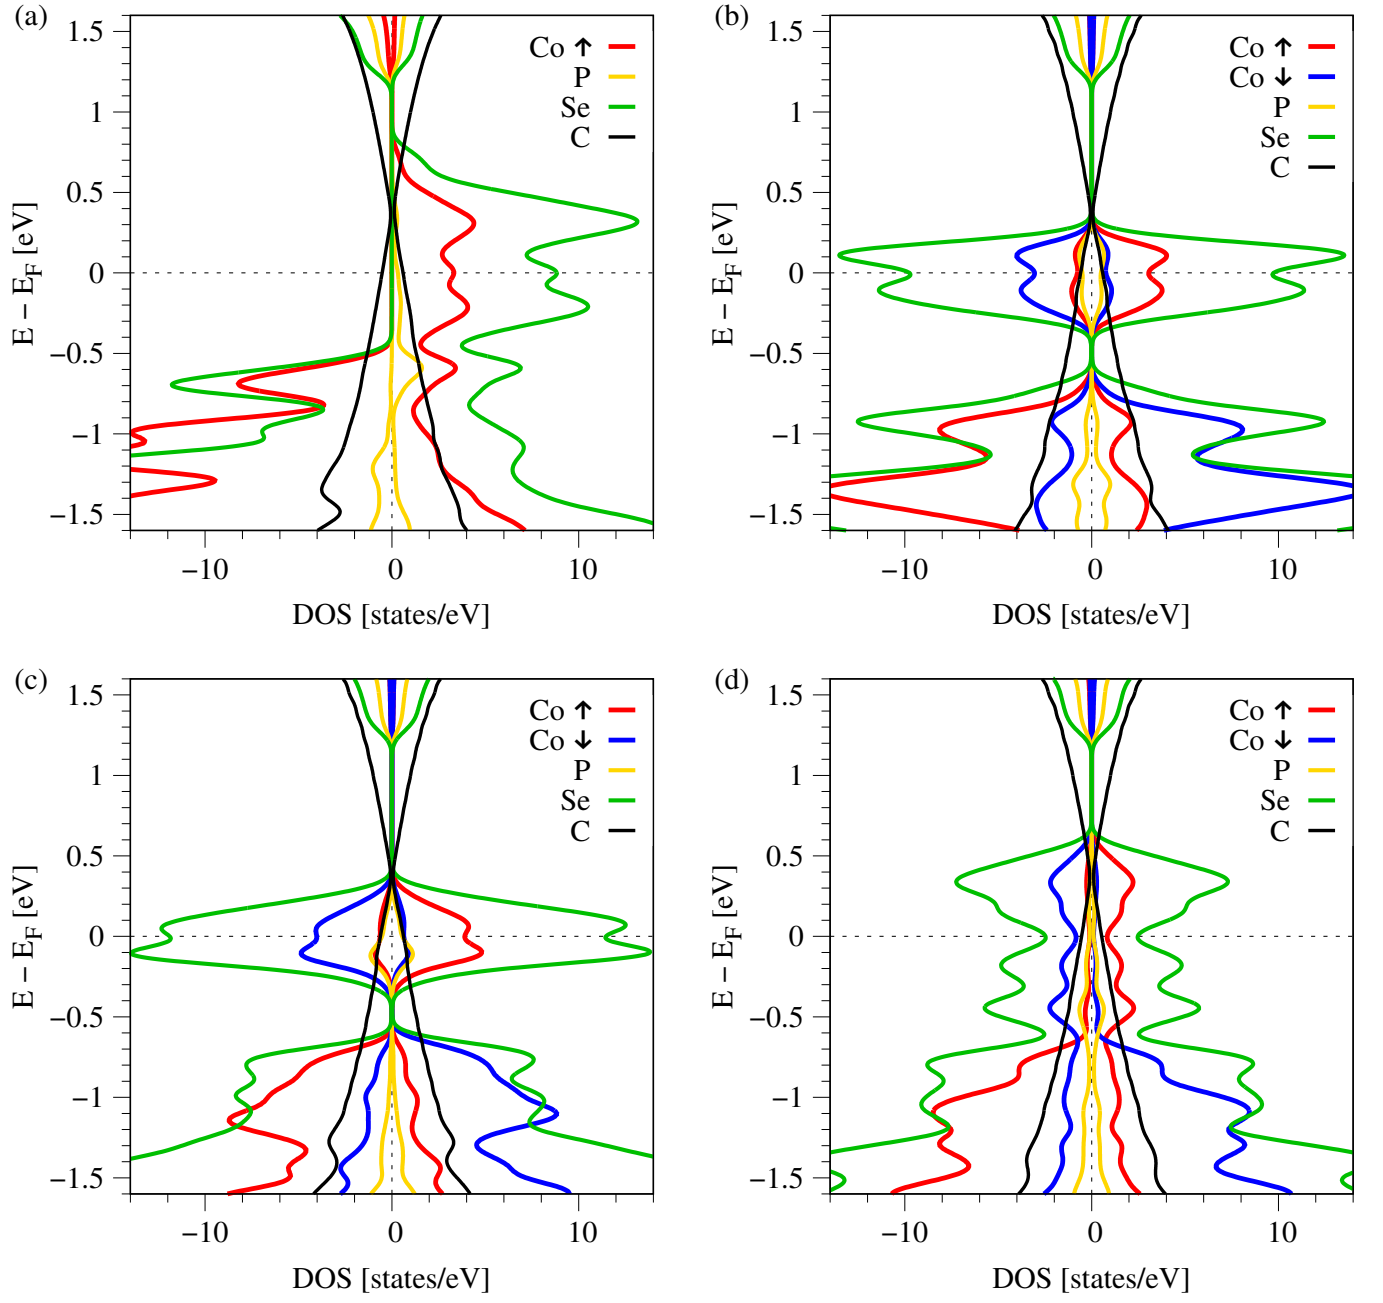

FIG. S31. Spin and atom resolved Density of States (DOS) for graphene on CoPSe<sub>3</sub> when CoPSe<sub>3</sub> is in the (a) ferromagnetic, (b) antiferromagnetic Néel, (c) antiferromagnetic zigzag, or (d) antiferromagnetic stripy phase.

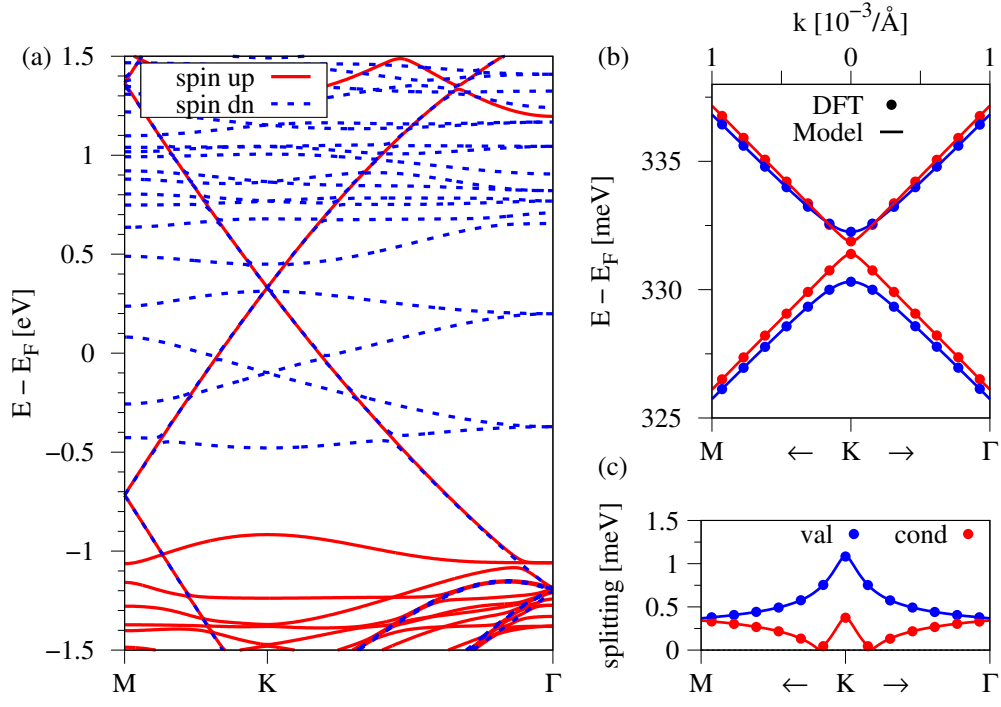

FIG. S32. (a) DFT-calculated band structure of the **graphene/FePS<sub>3</sub>** heterostructure along the high-symmetry path M-K- $\Gamma$  without SOC, when the FePS<sub>3</sub> is in the **ferromagnetic phase**. Red solid (blue dashed) lines correspond to spin up (spin down). (b) Zoom to the DFT-calculated (symbols) low energy Dirac bands near the K point with a fit to the model Hamiltonian (solid line). (c) The splitting of valence and conduction band.

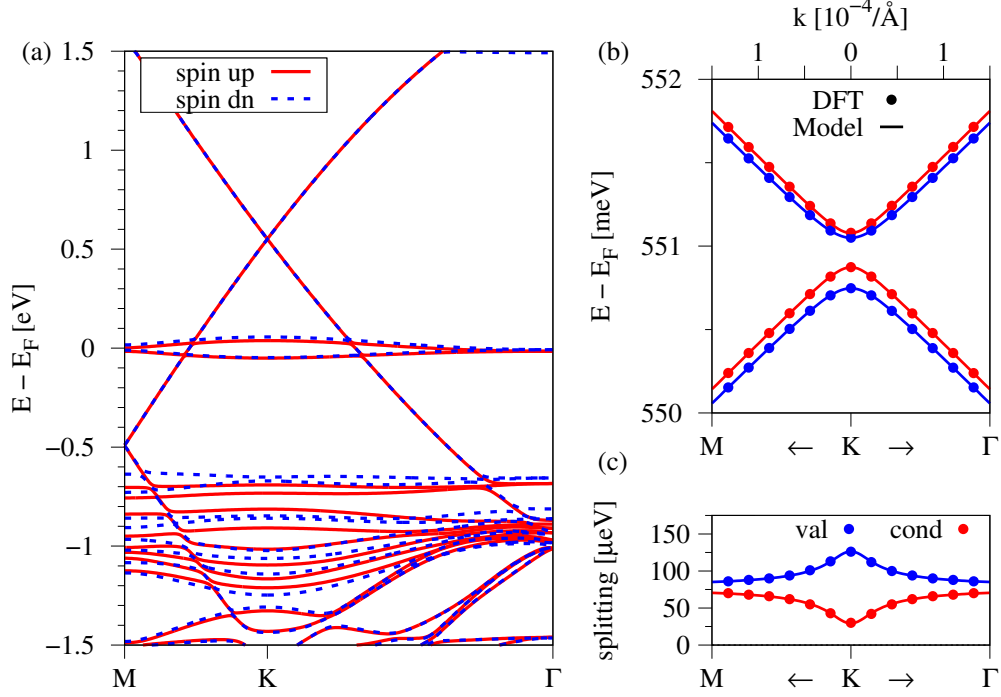

FIG. S33. (a) DFT-calculated band structure of the **graphene/FePS<sub>3</sub>** heterostructure along the high-symmetry path M-K- $\Gamma$  without SOC, when the FePS<sub>3</sub> is in the **antiferromagnetic Néel phase**. Red solid (blue dashed) lines correspond to spin up (spin down). (b) Zoom to the DFT-calculated (symbols) low energy Dirac bands near the K point with a fit to the model Hamiltonian (solid line). (c) The splitting of valence and conduction band.

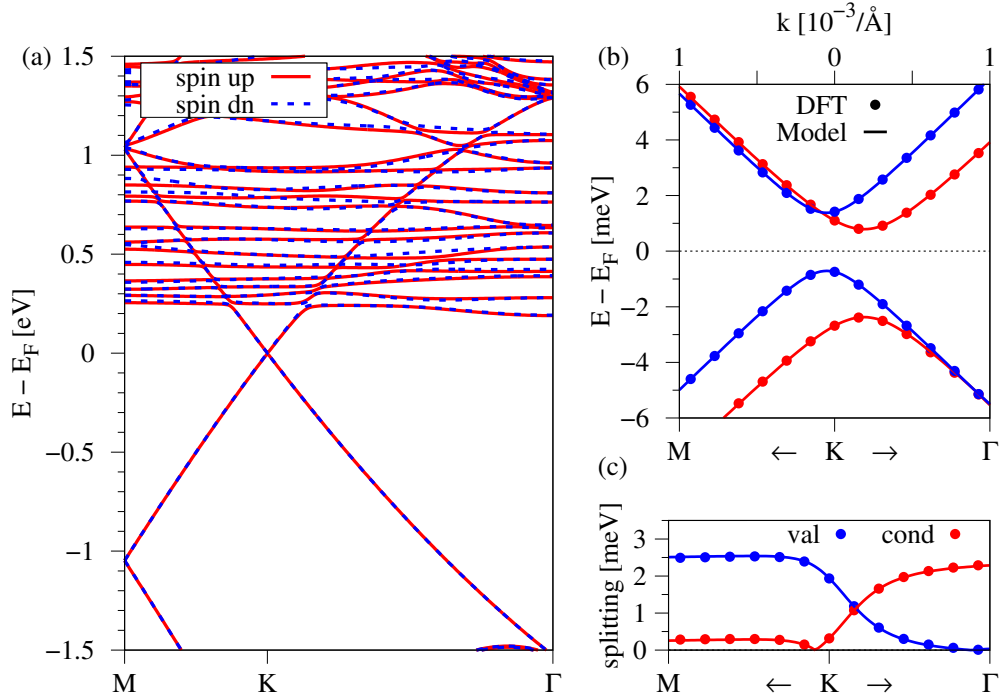

FIG. S34. (a) DFT-calculated band structure of the **graphene/FePS<sub>3</sub>** heterostructure along the high-symmetry path M-K- $\Gamma$  without SOC, when the FePS<sub>3</sub> is in the **antiferromagnetic zigzag phase**. Red solid (blue dashed) lines correspond to spin up (spin down). (b) Zoom to the DFT-calculated (symbols) low energy Dirac bands near the K point with a fit to the model Hamiltonian (solid line). (c) The splitting of valence and conduction band.

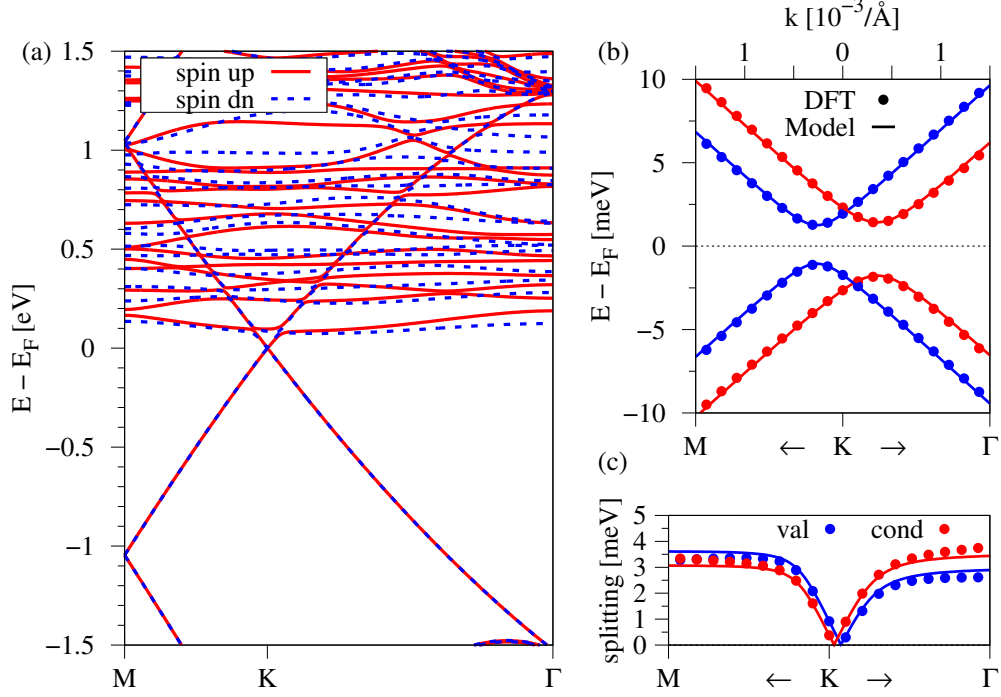

FIG. S35. (a) DFT-calculated band structure of the **graphene/FePS<sub>3</sub>** heterostructure along the high-symmetry path M-K- $\Gamma$  without SOC, when the FePS<sub>3</sub> is in the **antiferromagnetic stripy phase**. Red solid (blue dashed) lines correspond to spin up (spin down). (b) Zoom to the DFT-calculated (symbols) low energy Dirac bands near the K point with a fit to the model Hamiltonian (solid line). (c) The splitting of valence and conduction band.

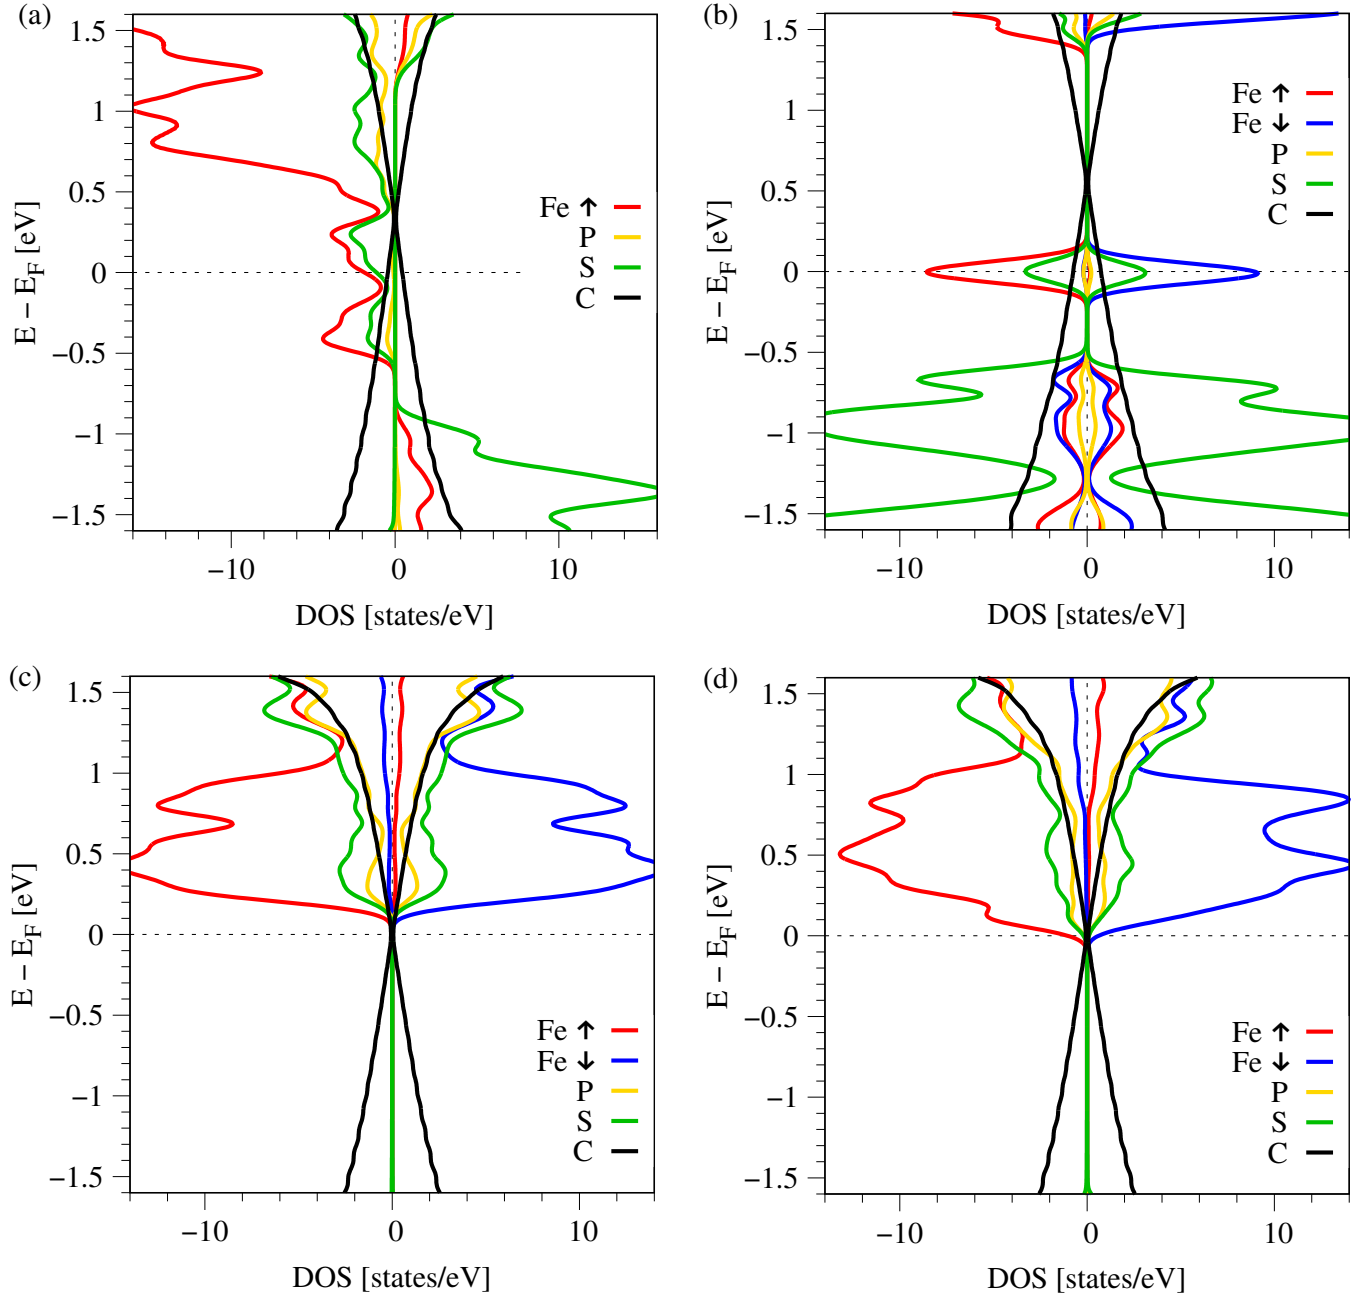

FIG. S36. Spin and atom resolved Density of States (DOS) for graphene on FePS<sub>3</sub> when FePS<sub>3</sub> is in the (a) ferromagnetic, (b) antiferromagnetic Néel, (c) antiferromagnetic zigzag, or (d) antiferromagnetic stripy phase.



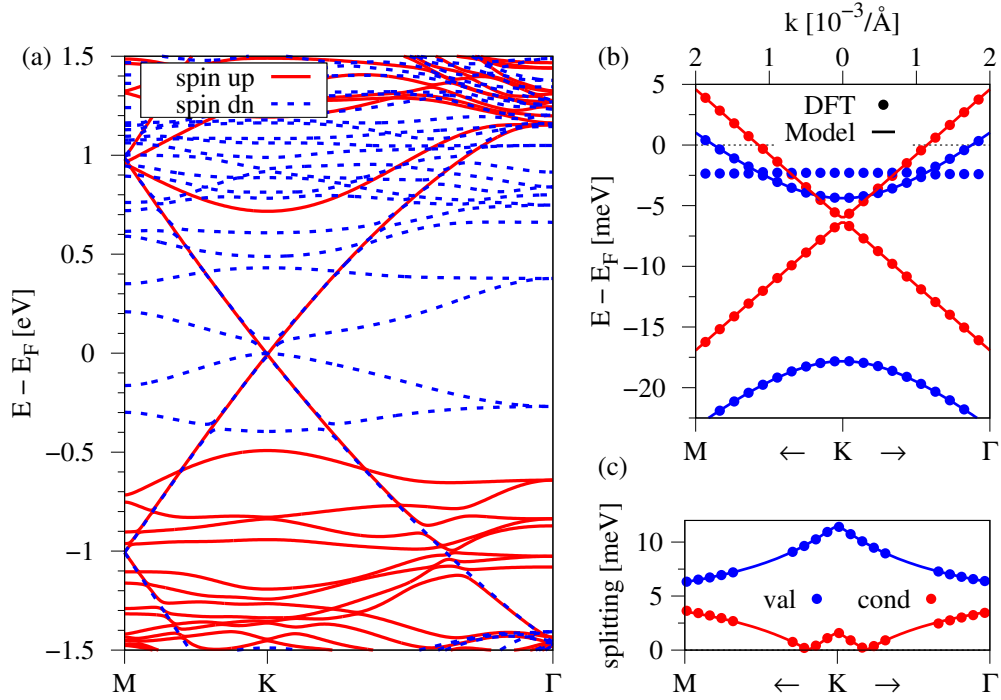

FIG. S37. (a) DFT-calculated band structure of the **graphene/FePSe<sub>3</sub>** heterostructure along the high-symmetry path M-K- $\Gamma$  without SOC, when the FePSe<sub>3</sub> is in the **ferromagnetic phase**. Red solid (blue dashed) lines correspond to spin up (spin down). (b) Zoom to the DFT-calculated (symbols) low energy Dirac bands near the K point with a fit to the model Hamiltonian (solid line). (c) The splitting of valence and conduction band.

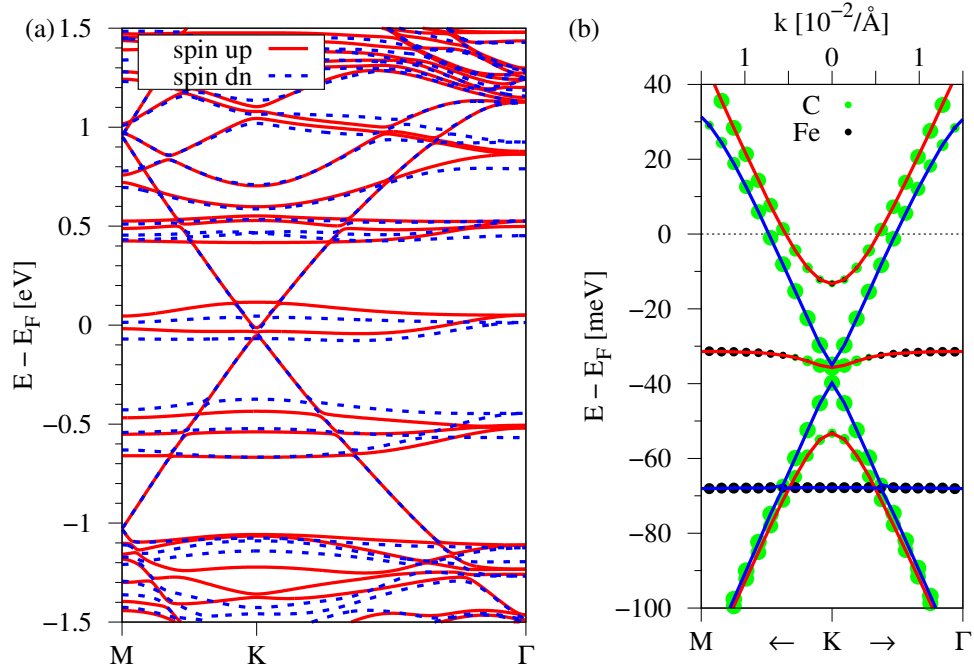

FIG. S38. (a) DFT-calculated band structure of the **graphene/FePSe<sub>3</sub>** heterostructure along the high-symmetry path M-K- $\Gamma$  without SOC, when the FePSe<sub>3</sub> is in the **antiferromagnetic Néel phase**. Red solid (blue dashed) lines correspond to spin up (spin down). (b) Zoom to the DFT-calculated (symbols) low energy Dirac bands near the K point with a fit to the model Hamiltonian (solid line). (c) The splitting of valence and conduction band.

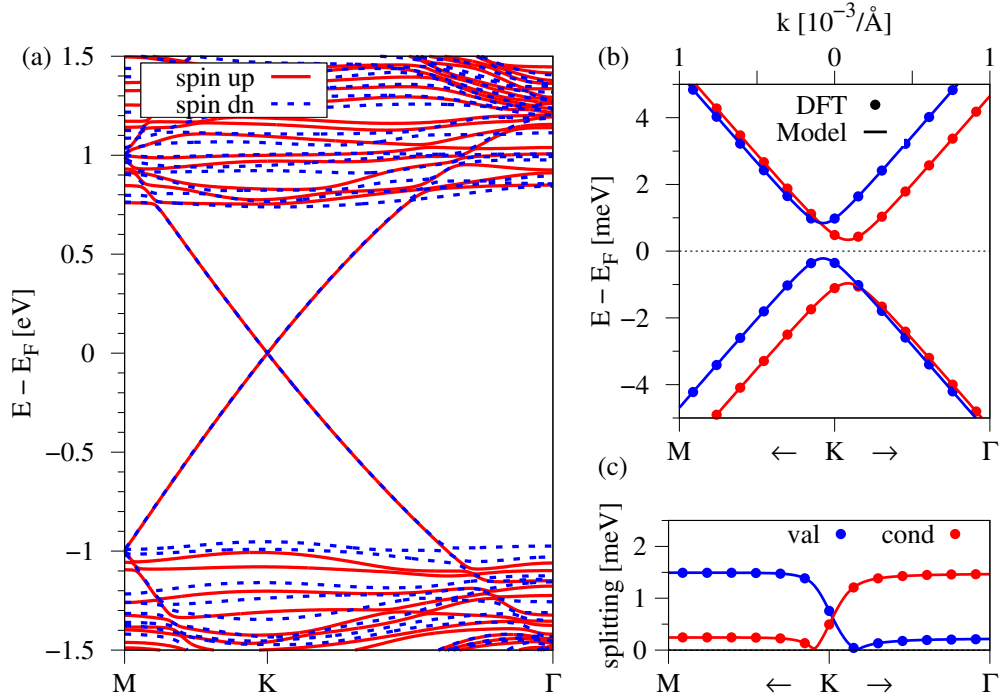

FIG. S39. (a) DFT-calculated band structure of the **graphene/FePSe<sub>3</sub>** heterostructure along the high-symmetry path M-K- $\Gamma$  without SOC, when the FePSe<sub>3</sub> is in the **antiferromagnetic zigzag phase**. Red solid (blue dashed) lines correspond to spin up (spin down). (b) Zoom to the DFT-calculated (symbols) low energy Dirac bands near the K point with a fit to the model Hamiltonian (solid line). (c) The splitting of valence and conduction band.

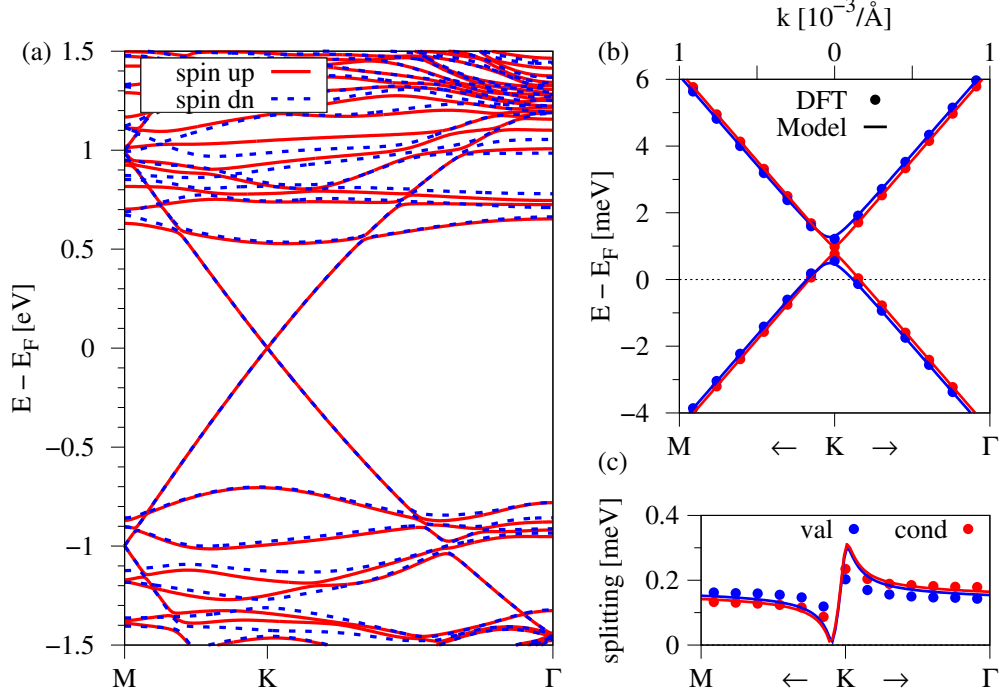

FIG. S40. (a) DFT-calculated band structure of the **graphene/FePSe<sub>3</sub>** heterostructure along the high-symmetry path M-K- $\Gamma$  without SOC, when the FePSe<sub>3</sub> is in the **antiferromagnetic stripy phase**. Red solid (blue dashed) lines correspond to spin up (spin down). (b) Zoom to the DFT-calculated (symbols) low energy Dirac bands near the K point with a fit to the model Hamiltonian (solid line). (c) The splitting of valence and conduction band.

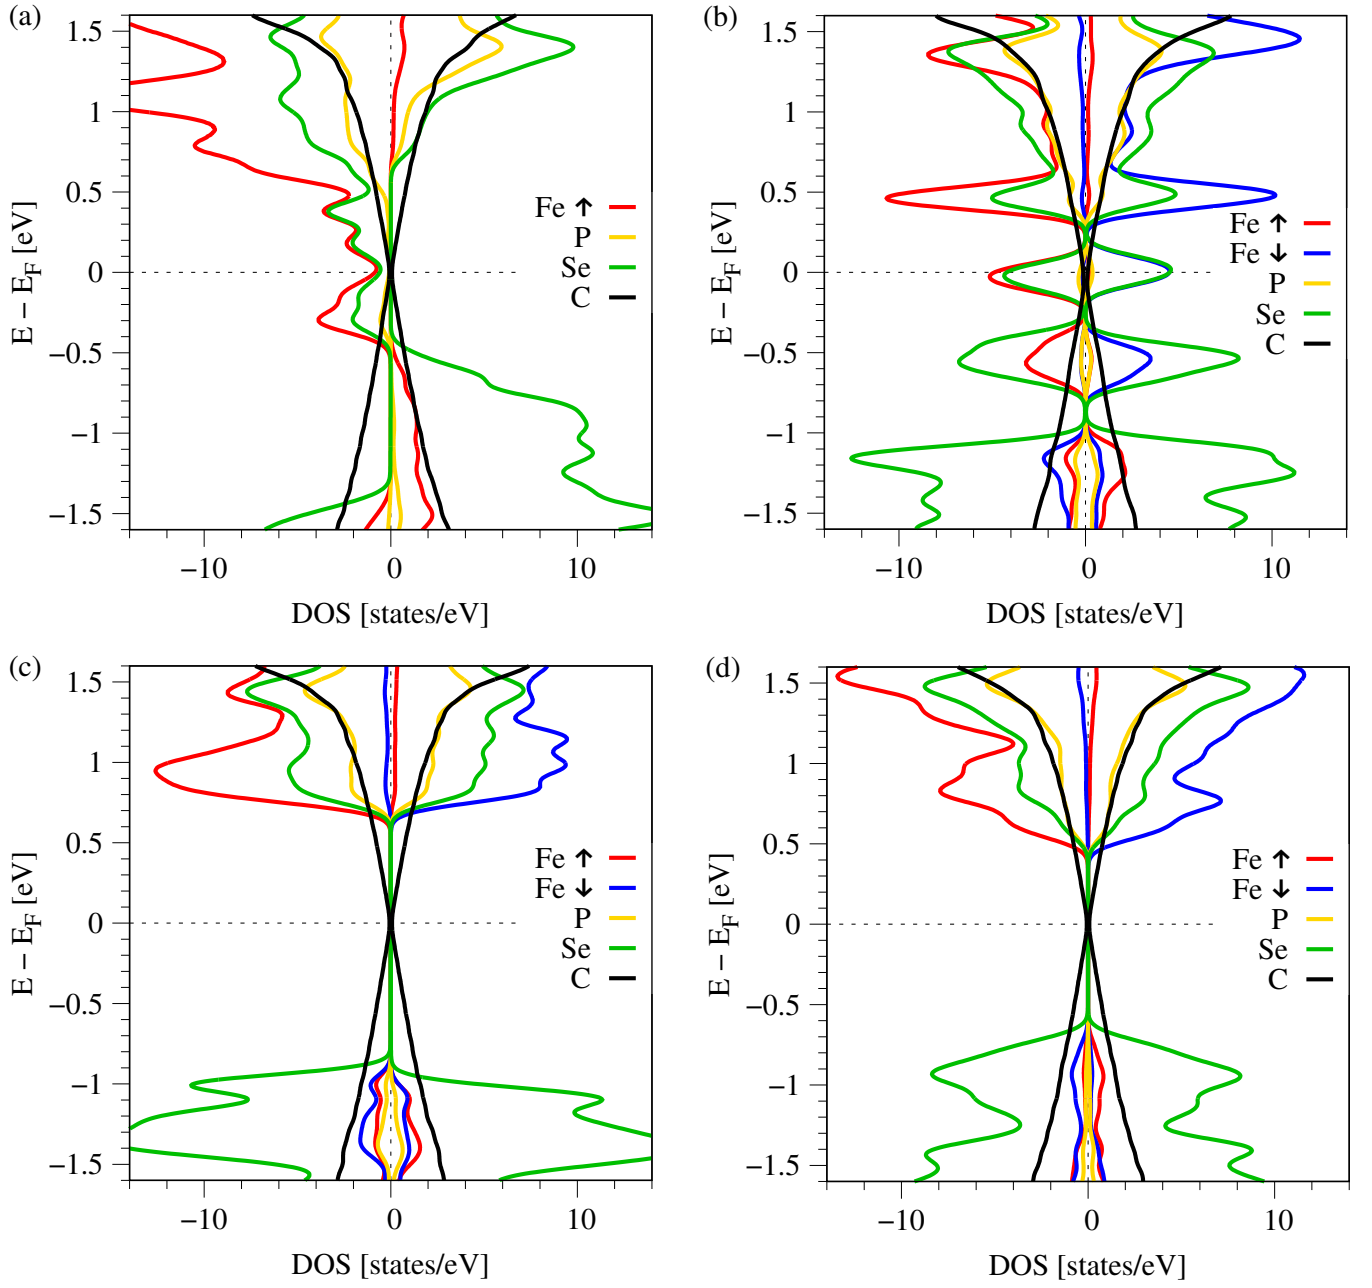

FIG. S41. Spin and atom resolved Density of States (DOS) for graphene on FePSe<sub>3</sub> when FePSe<sub>3</sub> is in the (a) ferromagnetic, (b) antiferromagnetic Néel, (c) antiferromagnetic zigzag phase, or (d) antiferromagnetic stripy phase.
